# Supplementary material for: More elementary components of the Hilbert scheme of points
Source: arXiv:2102.00494 ancillary file (2022-08-29)
Supplement: Supplementary file 1 [file signature_3,4,6,2,1.pdf]

# Signature (3, 4, 6, 2, 1).

In this notebook we construct the generic modification of the generic distinguished ideal of signature (3, 4, 6, 2, 1) (and Hilbert function (1, 3, 6, 10, 3, 3, 3)), and verify that it is an  $O$ -border basis; this is Example 8.1.1 in the paper.

**Note:** To execute this file, the notebook titled *utility functions for paper.nb* must be executed first.

---

## Set up the example with signature (3, 4, 6, 2, 1).

```
In[ ]:= n = 3;  
varList = Table[xi, {i, 1, n}]
```

```
Out[ ]:= {x1, x2, x3}
```

The next function **makeBasisAndBoundaryMonomialLists** computes and returns the lists of basis and boundary monomials, the Hilbert function  $H$ , the leading monomials  $LM$ , the trailing monomials  $TM$ , the sets  $\mathcal{T}' = \text{TarPrime}$  and  $\mathcal{T} = \text{Tar}$ , and the parameters

$\mu = |\text{basis}|$ ,  $\nu = |\text{bdry}|$ ,  $\ell = |LM|$ , and  $\tau = |TM|$ . The inputs are the components of the signature  $(n, r, s, \delta, w)$ . This function is defined in the notebook *utility functions for paper.nb*.

```
In[ ]:= {basis, bdry, H, LM, TM, tarPrime, tar,  $\mu$ ,  $\nu$ ,  $\ell$ ,  $\tau$ } =  
makeBasisAndBoundaryMonomialLists[n, r = 4, s = 6,  $\delta$  = 2, w = 1];
```

```
In[ ]:= basis
```

```
Out[ ]:= {1, x1, x2, x3, x12, x1x2, x1x3, x22, x2x3, x32, x13, x12x2, x12x3, x1x22, x1x2x3,  
x1x32, x23, x22x3, x2x32, x33, x22x32, x2x33, x34, x22x33, x2x34, x35, x22x34, x2x35, x36}
```

```
In[ ]:= bdry
```

```
Out[ ]:= {x14, x13x2, x13x3, x12x22, x12x2x3, x12x32, x1x23, x1x22x3, x1x2x32, x1x33, x24, x23x3, x1x22x32, x1x2x33,  
x1x34, x23x32, x1x22x33, x1x2x34, x1x35, x23x33, x1x22x34, x1x2x35, x1x36, x23x34, x22x35, x2x36, x37}
```

```
In[ ]:= H
```

```
Out[ ]:= {1, 3, 6, 10, 3, 3, 3}
```

```
In[ ]:= LM
```

```
Out[ ]:= {x14, x13x2, x13x3, x12x22, x12x2x3, x12x32, x1x23, x1x22x3, x1x2x32, x1x33, x24, x23x3}
```

```
In[ ]:= TM
```

```
Out[ ]:= {x22x34, x2x35, x36}
```

```
In[ ]:= tarPrime
```

```
Out[ ]:= {x2^2 x3^2, x2 x3^3, x3^4, x2^2 x3^3, x2 x3^4, x3^5}
```

```
In[ ]:= tar
```

```
Out[ ]:= {x2^2 x3^2, x2 x3^3, x3^4, x2^2 x3^3, x2 x3^4, x3^5, x2^2 x3^4, x2 x3^5, x3^6}
```

```
In[ ]:= {μ, ν, ℓ, τ}
```

```
Out[ ]:= {29, 27, 12, 3}
```

Next we compute the parameters  $\gamma$  and  $\eta$ , the set of initial target monomials (of which there are  $\gamma$ ), and the dimension of the affine space  $U$ .

```
In[ ]:= γ = numThetas[n, r, s, δ, w]
```

```
Out[ ]:= 6
```

```
In[ ]:= η = findEta[n, r, s, δ, w]
```

```
Out[ ]:= 6
```

```
In[ ]:= initialTargetMons[tarPrime, n, δ, w]
```

```
Out[ ]:= {x2^2 x3^2, x2 x3^3, x3^4, x2^2 x3^3, x2 x3^4, x3^5}
```

The next function returns the dimension of the affine space  $U$ . The formula used is equation (54) in the paper. The implementation is found in the utilities notebook.

```
In[ ]:= findDimU[n, r, s, δ, w, ℓ, τ]
```

```
Out[ ]:= 50
```

---

## Construct the border basis **genBorBasis**) of the generic distinguished ideal / of the given signature.

We first construct the generic generators associated to the leading monomials, after which we append the non-leading boundary monomials.

```
In[ ]:= borBasisA = Table[bdry[[j]] - Sum[C[i,j] * TM[[i]], {j, 1, ℓ}]
```

```
Out[ ]:= {x1^4 - C_{1,1} x2^2 x3^4 - C_{2,1} x2 x3^5 - C_{3,1} x3^6, x1^3 x2 - C_{1,2} x2^2 x3^4 - C_{2,2} x2 x3^5 - C_{3,2} x3^6,
x1^3 x3 - C_{1,3} x2^2 x3^4 - C_{2,3} x2 x3^5 - C_{3,3} x3^6, x1^2 x2^2 - C_{1,4} x2^2 x3^4 - C_{2,4} x2 x3^5 - C_{3,4} x3^6,
x1^2 x2 x3 - C_{1,5} x2^2 x3^4 - C_{2,5} x2 x3^5 - C_{3,5} x3^6, x1^2 x3^2 - C_{1,6} x2^2 x3^4 - C_{2,6} x2 x3^5 - C_{3,6} x3^6,
x1 x2^3 - C_{1,7} x2^2 x3^4 - C_{2,7} x2 x3^5 - C_{3,7} x3^6, x1 x2^2 x3 - C_{1,8} x2^2 x3^4 - C_{2,8} x2 x3^5 - C_{3,8} x3^6,
x1 x2 x3^2 - C_{1,9} x2^2 x3^4 - C_{2,9} x2 x3^5 - C_{3,9} x3^6, x1 x3^3 - C_{1,10} x2^2 x3^4 - C_{2,10} x2 x3^5 - C_{3,10} x3^6,
x2^4 - C_{1,11} x2^2 x3^4 - C_{2,11} x2 x3^5 - C_{3,11} x3^6, x2^3 x3 - C_{1,12} x2^2 x3^4 - C_{2,12} x2 x3^5 - C_{3,12} x3^6}
```

```
In[ ]:= genBorBasis = Join[borBasisA, Take[bdry, -(v - l)]]
```

```
Out[ ]:= {x1^4 - C_{1,1} x2^2 x3^4 - C_{2,1} x2 x3^5 - C_{3,1} x3^6, x1^3 x2 - C_{1,2} x2^2 x3^4 - C_{2,2} x2 x3^5 - C_{3,2} x3^6,
x1^2 x3 - C_{1,3} x2^2 x3^4 - C_{2,3} x2 x3^5 - C_{3,3} x3^6, x1^2 x2^2 - C_{1,4} x2^2 x3^4 - C_{2,4} x2 x3^5 - C_{3,4} x3^6,
x1^2 x2 x3 - C_{1,5} x2^2 x3^4 - C_{2,5} x2 x3^5 - C_{3,5} x3^6, x1^2 x3^2 - C_{1,6} x2^2 x3^4 - C_{2,6} x2 x3^5 - C_{3,6} x3^6,
x1 x2^3 - C_{1,7} x2^2 x3^4 - C_{2,7} x2 x3^5 - C_{3,7} x3^6, x1 x2^2 x3 - C_{1,8} x2^2 x3^4 - C_{2,8} x2 x3^5 - C_{3,8} x3^6,
x1 x2 x3^2 - C_{1,9} x2^2 x3^4 - C_{2,9} x2 x3^5 - C_{3,9} x3^6, x1 x3^3 - C_{1,10} x2^2 x3^4 - C_{2,10} x2 x3^5 - C_{3,10} x3^6,
x2^4 - C_{1,11} x2^2 x3^4 - C_{2,11} x2 x3^5 - C_{3,11} x3^6, x2^3 x3 - C_{1,12} x2^2 x3^4 - C_{2,12} x2 x3^5 - C_{3,12} x3^6, x1 x2^2 x3^2,
x1 x2 x3^3, x1 x3^4, x2^3 x3^2, x1 x2^2 x3^3, x1 x2 x3^4, x1 x3^5, x2^3 x3^3, x1 x2^2 x3^4, x1 x2 x3^5, x1 x3^6, x2^3 x3^4, x2^2 x3^5, x2 x3^6, x3^7}
```

## Build the generic modification of genBorBasis.

Following example 8.1.1 in the paper, we construct the generic modification of genBorBasis. As shown in the example, we need to add the generic target  $Y(b_{j_k})$  to borBasis[[k]] for

$b_{j_0} = b_{11} = x_2^4$ ,  $b_{j_1} = b_{12} = x_2^3 x_3$ ,  $b_{j_2} = b_{16} = x_2^3 x_3^2$ , and  $b_{j_3} = b_{20} = x_2^3 x_3^3$ . The generic target function is given by

```
In[ ]:= Y[b_] := 0; (* The value 0 is returned for all inputs other than 11, 12, 16, and 20. *)
Y[12] = x2^2 x3^2 theta1 + x2 x3^3 theta2 + x3^4 theta3 + x2^2 x3^3 theta4 + x2 x3^4 theta5 + x3^5 theta6;
Y[16] = x2^2 x3^3 theta1 + x2 x3^4 theta2 + x3^5 theta3 + x2^2 x3^4 theta4 + x2 x3^5 theta5 + x3^6 theta6;
Y[20] = x2^2 x3^4 theta1 + x2 x3^5 theta2 + x3^6 theta3;
Y[11] = (theta2 - theta1^2) (x2^2 x3^2) + (theta3 - theta1 theta2) x2 x3^3 + (-theta1 theta3) x3^4 +
(theta5 - 2 theta1 theta4) x2^2 x3^3 + (-theta2 theta4 - theta1 theta5 + theta6) x2 x3^4 + (-theta3 theta4 - theta1 theta6) x3^5;
```

```
In[ ]:= modGenBorBasis = Table[genBorBasis[[j]] + Y[j], {j, 1, v}]
```

```
Out[ ]:= {x1^4 - C_{1,1} x2^2 x3^4 - C_{2,1} x2 x3^5 - C_{3,1} x3^6, x1^3 x2 - C_{1,2} x2^2 x3^4 - C_{2,2} x2 x3^5 - C_{3,2} x3^6,
x1^2 x3 - C_{1,3} x2^2 x3^4 - C_{2,3} x2 x3^5 - C_{3,3} x3^6, x1^2 x2^2 - C_{1,4} x2^2 x3^4 - C_{2,4} x2 x3^5 - C_{3,4} x3^6,
x1^2 x2 x3 - C_{1,5} x2^2 x3^4 - C_{2,5} x2 x3^5 - C_{3,5} x3^6, x1^2 x3^2 - C_{1,6} x2^2 x3^4 - C_{2,6} x2 x3^5 - C_{3,6} x3^6,
x1 x2^3 - C_{1,7} x2^2 x3^4 - C_{2,7} x2 x3^5 - C_{3,7} x3^6, x1 x2^2 x3 - C_{1,8} x2^2 x3^4 - C_{2,8} x2 x3^5 - C_{3,8} x3^6,
x1 x2 x3^2 - C_{1,9} x2^2 x3^4 - C_{2,9} x2 x3^5 - C_{3,9} x3^6, x1 x3^3 - C_{1,10} x2^2 x3^4 - C_{2,10} x2 x3^5 - C_{3,10} x3^6,
x2^4 - C_{1,11} x2^2 x3^4 - C_{2,11} x2 x3^5 - C_{3,11} x3^6 + x2^2 x3^3 (-theta1^2 + theta2) - x3^4 theta1 theta3 +
x2 x3^3 (-theta1 theta2 + theta3) + x2^2 x3^3 (-2 theta1 theta4 + theta5) + x2 x3^4 (-theta2 theta4 - theta1 theta5 + theta6) + x3^5 (-theta3 theta4 - theta1 theta6),
x2^3 x3 - C_{1,12} x2^2 x3^4 - C_{2,12} x2 x3^5 - C_{3,12} x3^6 + x2^2 x3^3 theta1 + x2 x3^3 theta2 + x3^4 theta3 + x2^2 x3^3 theta4 + x2 x3^4 theta5 + x3^5 theta6,
x1 x2^2 x3^2, x1 x2 x3^3, x1 x3^4, x2^3 x3^2 + x2^2 x3^3 theta1 + x2 x3^4 theta2 + x3^5 theta3 + x2^2 x3^4 theta4 + x2 x3^5 theta5 + x3^6 theta6, x1 x2^2 x3^3,
x1 x2 x3^4, x1 x3^5, x2^3 x3^3 + x2^2 x3^4 theta1 + x2 x3^5 theta2 + x3^6 theta3, x1 x2^2 x3^4, x1 x2 x3^5, x1 x3^6, x2^3 x3^4, x2^2 x3^5, x2 x3^6, x3^7}
```

## Find the generators of the border basis scheme for the given order ideal “basis.”

```
In[ ]:= borBasisIdealGens = makeBorBasisSchemeIdealGenerators[basis, varList];
```

```
In[ ]:= borBasisIdealGens [ [2] ]
```

```
Out[ ]:= -C_{2,3} C_{11,26} + C_{2,2} C_{11,27} - C_{2,5} C_{12,26} + C_{2,4} C_{12,27} - C_{2,6} C_{13,26} + C_{2,5} C_{13,27} -  
C_{2,8} C_{14,26} + C_{2,7} C_{14,27} - C_{2,9} C_{15,26} + C_{2,8} C_{15,27} - C_{2,10} C_{16,26} + C_{2,9} C_{16,27} -  
C_{2,12} C_{17,26} + C_{2,11} C_{17,27} + C_{2,12} C_{18,27} + C_{2,16} C_{21,27} + C_{2,20} C_{24,27} -  
C_{2,25} C_{27,26} + C_{2,24} C_{27,27} - C_{2,26} C_{28,26} + C_{2,25} C_{28,27} - C_{2,27} C_{29,26} + C_{2,26} C_{29,27}
```

```
In[ ]:= Length [borBasisIdealGens]
```

```
Out[ ]:= 1305
```

## Confirm that modGenBorBasis is a border basis for the order ideal “basis.”

To do this, we first make the list of substitutions  $C_{\{i,j\}} \rightarrow c_{ij}$ , where the coefficient of  $t_i$  in the ideal generator with leading monomial  $b_j$  is  $-c_{ij}$ . That is, the  $c_{ij} = Y_{ij}$  are the generic modification coefficients as in section 10.1 of the “More elementary components” paper.

```
In[ ]:= 1stOfCSubs = makeCCoordsOfBorBasis [modGenBorBasis, basis, bdry, varList];
```

```
In[ ]:= Length [1stOfCSubs]
```

```
Out[ ]:= 783
```

The number of elements in the list should equal  $\mu v$ ; let's check:

```
In[ ]:=  $\mu v$ 
```

```
Out[ ]:= 783
```

Now we substitute the generic modification coefficients into the polynomials in borBasisIdealGens, and show that all of them reduce to 0:

```
In[ ]:= DeleteDuplicates [Expand [borBasisIdealGens /. 1stOfCSubs]]
```

```
Out[ ]:= {0}
```

## Find the tangent space dimension at a randomly-chosen mod-distinguished ideal.

We first construct our mod-distinguished ideal by assigning random scalar values to the distinguished  $C_{\{i,j\}}$  and the  $\theta_k$ .

Recall that the distinguished  $C_{\{i,j\}}$  are such that  $t_i \in \text{TM}$  and  $b_j \in \text{LM}$ , so  $1 \leq i \leq \ell = \mu$ , and  $25 \leq j \leq v = 27$ .

```
In[*]:= distCLst = Flatten[Table[C{i,j}, {j, 25, v}, {i, 1, l}]]
```

```
Out[*]:= {C{1,25}, C{2,25}, C{3,25}, C{4,25}, C{5,25}, C{6,25}, C{7,25}, C{8,25}, C{9,25}, C{10,25}, C{11,25}, C{12,25},  
C{1,26}, C{2,26}, C{3,26}, C{4,26}, C{5,26}, C{6,26}, C{7,26}, C{8,26}, C{9,26}, C{10,26}, C{11,26}, C{12,26},  
C{1,27}, C{2,27}, C{3,27}, C{4,27}, C{5,27}, C{6,27}, C{7,27}, C{8,27}, C{9,27}, C{10,27}, C{11,27}, C{12,27}}
```

```
In[*]:= lstOfThetas = Table[θk, {k, 1, γ}]
```

```
Out[*]:= {θ1, θ2, θ3, θ4, θ5, θ6}
```

```
In[*]:= distCSubLst = Table[distCLst[[i]] → RandomInteger[{-2, 2}], {i, 1, Length[distCLst]}]
```

```
Out[*]:= {C{1,25} → 0, C{2,25} → 2, C{3,25} → -1, C{4,25} → -2, C{5,25} → 2, C{6,25} → 2, C{7,25} → 2, C{8,25} → -2,  
C{9,25} → 1, C{10,25} → 1, C{11,25} → 1, C{12,25} → 2, C{1,26} → 0, C{2,26} → 0, C{3,26} → -1,  
C{4,26} → 2, C{5,26} → 0, C{6,26} → 2, C{7,26} → -1, C{8,26} → -1, C{9,26} → 2, C{10,26} → -1,  
C{11,26} → -2, C{12,26} → -1, C{1,27} → -2, C{2,27} → -2, C{3,27} → -1, C{4,27} → -2, C{5,27} → 0,  
C{6,27} → 1, C{7,27} → -1, C{8,27} → 2, C{9,27} → 1, C{10,27} → 1, C{11,27} → 0, C{12,27} → 2}
```

```
In[*]:= thetaSubLst = Table[lstOfThetas[[k]] → RandomInteger[{-2, 2}], {k, 1, Length[lstOfThetas]}]
```

```
Out[*]:= {θ1 → 2, θ2 → 2, θ3 → -1, θ4 → -1, θ5 → -1, θ6 → -1}
```

```
In[*]:= indetSubLst = Join[distCSubLst, thetaSubLst]
```

```
Out[*]:= {C{1,25} → 0, C{2,25} → 2, C{3,25} → -1, C{4,25} → -2, C{5,25} → 2, C{6,25} → 2, C{7,25} → 2,  
C{8,25} → -2, C{9,25} → 1, C{10,25} → 1, C{11,25} → 1, C{12,25} → 2, C{1,26} → 0, C{2,26} → 0,  
C{3,26} → -1, C{4,26} → 2, C{5,26} → 0, C{6,26} → 2, C{7,26} → -1, C{8,26} → -1, C{9,26} → 2,  
C{10,26} → -1, C{11,26} → -2, C{12,26} → -1, C{1,27} → -2, C{2,27} → -2, C{3,27} → -1,  
C{4,27} → -2, C{5,27} → 0, C{6,27} → 1, C{7,27} → -1, C{8,27} → 2, C{9,27} → 1, C{10,27} → 1,  
C{11,27} → 0, C{12,27} → 2, θ1 → 2, θ2 → 2, θ3 → -1, θ4 → -1, θ5 → -1, θ6 → -1}
```

```
In[*]:= modDistBorBasis = modGenBorBasis /. indetSubLst
```

```
Out[*]:= {x14 - C{1,1} x22 x34 - C{2,1} x2 x35 - C{3,1} x36, x13 x2 - C{1,2} x22 x34 - C{2,2} x2 x35 - C{3,2} x36,  
x13 x3 - C{1,3} x22 x34 - C{2,3} x2 x35 - C{3,3} x36, x12 x22 - C{1,4} x22 x34 - C{2,4} x2 x35 - C{3,4} x36,  
x12 x2 x3 - C{1,5} x22 x34 - C{2,5} x2 x35 - C{3,5} x36, x12 x32 - C{1,6} x22 x34 - C{2,6} x2 x35 - C{3,6} x36,  
x1 x23 - C{1,7} x22 x34 - C{2,7} x2 x35 - C{3,7} x36, x1 x22 x3 - C{1,8} x22 x34 - C{2,8} x2 x35 - C{3,8} x36,  
x1 x2 x32 - C{1,9} x22 x34 - C{2,9} x2 x35 - C{3,9} x36, x1 x33 - C{1,10} x22 x34 - C{2,10} x2 x35 - C{3,10} x36,  
x24 - 2 x22 x32 - 5 x2 x33 + 3 x22 x33 + 2 x34 + 3 x2 x34 - C{1,11} x22 x34 + x35 - C{2,11} x2 x35 - C{3,11} x36,  
x23 x3 + 2 x22 x32 + 2 x2 x33 - x22 x33 - x34 - x2 x34 - C{1,12} x22 x34 - x35 - C{2,12} x2 x35 - C{3,12} x36,  
x1 x22 x32, x1 x2 x33, x1 x34, x23 x32 + 2 x22 x33 + 2 x2 x34 - x22 x34 - x35 - x2 x35 - x36, x1 x22 x33, x1 x2 x34,  
x1 x35, x23 x33 + 2 x22 x34 + 2 x2 x35 - x36, x1 x22 x34, x1 x2 x35, x1 x36, x23 x34, x22 x35, x2 x36, x37}
```

Find the tangent space relations and the dimension of the tangent space at the point  $[I]$  corresponding to the mod-distinguished ideal  $I = (\text{modDistBorBasis})$ .

We compute the tangent space dimension by first computing the “tangent space relations,” as explained in the previous paper “Some elementary components of the Hilbert scheme of points.”

```
In[*]:= {aLst, allTanSpaceReIns} = makeTanSpaceReIns[modDistBorBasis, basis, bdry, varList];
```

```
In[ ]:= aLstLength = Length[aLst]
```

```
Out[ ]:= 783
```

**Warning:** the following computation takes several minutes; it involves computing the rank of a very large matrix.

```
In[ ]:= tanSpaceDim[Length[aLst], allTanSpaceReIns]
```

```
Out[ ]:= 129
```

The computation would take less time if all the thetas had been set equal to 0 instead of to random values as above; the tangent space dimension turns out to be 129 in either case (assuming the distinguished  $C_{\{i,j\}}$  are sufficiently general) .

Note that the tangent space dimension is much larger than  $\dim(U) = 50$ , so we have not found an elementary component.

The principal component in this case has dimension:

```
In[ ]:=  $\mu * \tau$ 
```

```
Out[ ]:= 87
```
