# Supplementary material for: More elementary components of the Hilbert scheme of points
Source: arXiv:2102.00494 ancillary file (2022-08-29)
Supplement: Supplementary file 2 [file signature_5,2,3,3,0.pdf]

# Signature (5, 2, 3, 3, 0) and Hilbert function (1, 5, 5, 7).

Sufficiently general distinguished ideals of this signature are smooth points on an elementary component of dimension 86. The principal component has dimension  $5 \cdot 18 = 90$ .

**Note:** To execute this file, the notebook titled *utility functions for paper.nb* must be executed first.

---

## Set up the example.

```
In[ ]:= n = 5;  
varList = Table[xi, {i, 1, n}]
```

```
Out[ ]:= {x1, x2, x3, x4, x5}
```

The next function **makeBasisAndBoundaryMonomialLists** computes and returns the lists of basis and boundary monomials, the Hilbert function, the leading monomials LM, the trailing monomials TM, the sets  $\mathcal{T}' = \text{TarPrime}$  and  $\mathcal{T} = \text{Tar}$ , and the parameters

$\mu = |\text{basis}|$ ,  $\nu = |\text{bdry}|$ ,  $\ell = |\text{LM}|$ , and  $\tau = |\text{TM}|$ . This function is defined in the notebook *Utilities for modification construction 2020.nb*.

```
In[ ]:= {basis, bdry, H, LM, TM, tarPrime, tar,  $\mu$ ,  $\nu$ ,  $\ell$ ,  $\tau$ } =  
makeBasisAndBoundaryMonomialLists[n, r = 2, s = 3,  $\delta$  = 3, w = 0];
```

```
In[ ]:= basis
```

```
Out[ ]:= {1, x1, x2, x3, x4, x5, x3 x4, x3 x5, x42, x4 x5, x52, x3 x42, x3 x4 x5, x3 x52, x43, x42 x5, x4 x52, x53}
```

```
In[ ]:= bdry
```

```
Out[ ]:= {x12, x1 x2, x1 x3, x1 x4, x1 x5, x22, x2 x3, x2 x4, x2 x5, x32, x1 x3 x4, x1 x3 x5, x1 x42, x1 x4 x5,  
x1 x52, x2 x3 x4, x2 x3 x5, x2 x42, x2 x4 x5, x2 x52, x32 x4, x32 x5, x1 x3 x42, x1 x3 x4 x5, x1 x3 x52,  
x1 x43, x1 x42 x5, x1 x4 x52, x1 x53, x2 x3 x42, x2 x3 x4 x5, x2 x3 x52, x2 x43, x2 x42 x5, x2 x4 x52,  
x2 x53, x32 x42, x32 x4 x5, x32 x52, x3 x43, x3 x42 x5, x3 x4 x52, x3 x53, x44, x43 x5, x42 x52, x4 x53, x54}
```

```
In[ ]:= H
```

```
Out[ ]:= {1, 5, 5, 7}
```

```
In[ ]:= LM
```

```
Out[ ]:= {x12, x1 x2, x1 x3, x1 x4, x1 x5, x22, x2 x3, x2 x4, x2 x5, x32}
```

```
In[ ]:= TM
```

```
Out[ ]:= {x3 x4^2, x3 x4 x5, x3 x5^2, x4^3, x4^2 x5, x4 x5^2, x5^3}
```

```
In[ ]:= 1 * τ
```

```
Out[ ]:= 70
```

```
In[ ]:= n * μ
```

```
Out[ ]:= 90
```

```
In[ ]:= findDimU[n, r, s, δ, w, l, τ]
```

```
Out[ ]:= 86
```

Construct the border basis (**borBasis**) of a random distinguished ideal  $I$  of the given signature, and compute the dimension of the tangent space at  $[I] \in H$ .

We first compute the generators associated to the leading monomials, after which we append the non-leading boundary monomials.

```
In[ ]:= borBasisA = Table[bdry[[j]] - Sum[RandomInteger[{-1, 1}] * TM[[i]], {j, 1, l}]
```

```
Out[ ]:= {x1^2 - x3 x5^2 - x4 x5^2, x1 x2 + x4^3 - x3 x5^2 - x4 x5^2 - x5^3, x1 x3 - x3 x4^2 - x4^3 + x4^2 x5 - x3 x5^2,
  x1 x4 + x3 x4^2 + x3 x4 x5 - x4^2 x5 + x5^3, x1 x5 + x5^3, x2^2 + x4^3 - x3 x4 x5 + x4^2 x5 + x3 x5^2 + x4 x5^2 + x5^3,
  x2 x3 + x3 x4 x5 + x3 x5^2 + x4 x5^2, x2 x4 + x3 x4^2 - x4^3 - x4^2 x5 + x3 x5^2 - x4 x5^2 - x5^3,
  -x3 x4^2 - x4^3 + x2 x5 + x3 x4 x5 - x4 x5^2 + x5^3, x3^2 - x4^3 - x3 x4 x5 - x4^2 x5 + x3 x5^2 - x4 x5^2 + x5^3}
```

```
In[ ]:= borBasis = Join[borBasisA, Take[bdry, -(v - l)]]
```

```
Out[ ]:= {x1^2 - x3 x5^2 - x4 x5^2, x1 x2 + x4^3 - x3 x5^2 - x4 x5^2 - x5^3, x1 x3 - x3 x4^2 - x4^3 + x4^2 x5 - x3 x5^2,
  x1 x4 + x3 x4^2 + x3 x4 x5 - x4^2 x5 + x5^3, x1 x5 + x5^3, x2^2 + x4^3 - x3 x4 x5 + x4^2 x5 + x3 x5^2 + x4 x5^2 + x5^3,
  x2 x3 + x3 x4 x5 + x3 x5^2 + x4 x5^2, x2 x4 + x3 x4^2 - x4^3 - x4^2 x5 + x3 x5^2 - x4 x5^2 - x5^3,
  -x3 x4^2 - x4^3 + x2 x5 + x3 x4 x5 - x4 x5^2 + x5^3, x3^2 - x4^3 - x3 x4 x5 - x4^2 x5 + x3 x5^2 - x4 x5^2 + x5^3, x1 x3 x4,
  x1 x3 x5, x1 x4^2, x1 x4 x5, x1 x5^2, x2 x3 x4, x2 x3 x5, x2 x4^2, x2 x4 x5, x2 x5^2, x3^2 x4, x3^2 x5, x1 x3 x4^2,
  x1 x3 x4 x5, x1 x3 x5^2, x1 x4^3, x1 x4^2 x5, x1 x4 x5^2, x1 x5^3, x2 x3 x4^2, x2 x3 x4 x5, x2 x3 x5^2, x2 x4^3, x2 x4^2 x5,
  x2 x4 x5^2, x2 x5^3, x3^2 x4^2, x3^2 x4 x5, x3^2 x5^2, x3 x4^3, x3 x4^2 x5, x3 x4 x5^2, x3 x5^3, x4^4, x4^3 x5, x4^2 x5^2, x4 x5^3, x5^4}
```

Find the tangent space relations and the dimension of the tangent space at  $[I]$

Tangent space dimension at the distinguished point:

```
In[ ]:= varList
```

```
Out[ ]:= {x1, x2, x3, x4, x5}
```

```
In[ ]:= {aLst, allTanSpaceReIns} = makeTanSpaceReIns[borBasis, basis, bdry, varList];
```

```
In[ ]:= aLstLength = Length[aLst]
```

```
Out[ ]:= 864
```

```
In[ ]:= tanSpaceDim[Length[aLst], allTanSpaceReIns]
```

```
Out[ ]:= 86
```

```
In[ ]:= findDimU[n, r, s,  $\delta$ , w,  $\ell$ ,  $\tau$ ]
```

```
Out[ ]:= 86
```

Since  $\dim(U) = 86 =$  tangent space dimension at  $[I]$ , we have that  $[I]$  is a smooth point on an elementary component of dimension 86.

The dimension of the principal component is:

```
In[ ]:=  $\mu * n$ 
```

```
Out[ ]:= 90
```
