# Supplementary material for: More elementary components of the Hilbert scheme of points
Source: arXiv:2102.00494 ancillary file (2022-08-29)
Supplement: Supplementary file 6 [file signature_6,2,4,4,0.pdf]

# Signature (6, 2, 4, 4, 0) and Hilbert function (1, 6, 5, 7, 9)

In this case, sufficiently general distinguished ideals of this signature (and Hilbert function (1, 6, 5, 7, 9)) are smooth points on an elementary component of dimension 186. The principal component has dimension  $6 \cdot 28 = 168$ .

**Note:** To execute this file, the notebook titled *utility functions for paper.nb* must be executed first.

---

## Set up the example.

```
In[ ]:= n = 6;  
varList = Table[xi, {i, 1, n}]  
Out[ ]:= {x1, x2, x3, x4, x5, x6}
```

The next function **makeBasisAndBoundaryMonomialLists** computes and returns the lists of basis and boundary monomials, the Hilbert function, the leading monomials LM, the trailing monomials TM, the sets  $\mathcal{T}' = \text{TarPrime}$  and  $\mathcal{T} = \text{Tar}$ , and the parameters

$\mu = |\text{basis}|$ ,  $\nu = |\text{bdry}|$ ,  $\ell = |\text{LM}|$ , and  $\tau = |\text{TM}|$ . This function is defined in the notebook *Utilities for modification construction 2020.nb*.

```
In[ ]:= {basis, bdry, H, LM, TM, tarPrime, tar,  $\mu$ ,  $\nu$ ,  $\ell$ ,  $\tau$ } =  
makeBasisAndBoundaryMonomialLists[n, r = 2, s = 4,  $\delta$  = 4, w = 0];
```

```
In[ ]:= basis
```

```
Out[ ]:= {1, x1, x2, x3, x4, x5, x6, x4 x5, x4 x6, x52, x5 x6, x62, x4 x52, x4 x5 x6, x4 x62,  
x53, x52 x6, x5 x62, x63, x4 x53, x4 x52 x6, x4 x5 x62, x4 x63, x54, x53 x6, x52 x62, x5 x63, x64}
```

```
In[ ]:= bdry
```

```
Out[ ]:= {x12, x1 x2, x1 x3, x1 x4, x1 x5, x1 x6, x22, x2 x3, x2 x4, x2 x5, x2 x6, x32, x3 x4, x3 x5,  
x3 x6, x42, x4 x5, x4 x6, x52, x5 x6, x62, x4 x52, x4 x5 x6, x4 x62,  
x53, x52 x6, x5 x62, x63, x4 x53, x4 x52 x6, x4 x5 x62, x4 x63, x54, x53 x6, x52 x62, x5 x63, x64,  
x2 x4 x5, x3 x4 x5, x3 x4 x6, x3 x52, x3 x5 x6, x3 x62, x42 x5, x42 x6, x1 x4 x52, x1 x4 x5 x6, x1 x4 x62,  
x1 x53, x1 x52 x6, x1 x5 x62, x1 x63, x2 x4 x52, x2 x4 x5 x6, x2 x4 x62, x2 x53, x2 x52 x6, x2 x5 x62,  
x2 x63, x3 x4 x52, x3 x4 x5 x6, x3 x4 x62, x3 x53, x3 x52 x6, x3 x5 x62, x3 x63, x42 x52, x42 x5 x6,  
x42 x62, x1 x4 x53, x1 x4 x52 x6, x1 x4 x5 x62, x1 x4 x63, x1 x53 x6, x1 x52 x62, x1 x5 x63, x1 x64,  
x2 x4 x53, x2 x4 x52 x6, x2 x4 x5 x62, x2 x4 x63, x2 x54, x2 x53 x6, x2 x52 x62, x2 x5 x63, x2 x64, x3 x4 x53,  
x3 x4 x52 x6, x3 x4 x5 x62, x3 x4 x63, x3 x54, x3 x53 x6, x3 x52 x62, x3 x5 x63, x3 x64, x42 x53, x42 x52 x6,  
x42 x5 x62, x42 x63, x4 x54, x4 x53 x6, x4 x52 x62, x4 x5 x63, x4 x64, x55, x54 x6, x53 x62, x52 x63, x5 x64, x65}
```

In[\*]:= **H**

Out[\*]:= {1, 6, 5, 7, 9}

In[\*]:= **LM**

Out[\*]:=  $\{x_1^2, x_1 x_2, x_1 x_3, x_1 x_4, x_1 x_5, x_1 x_6, x_2^2, x_2 x_3, x_2 x_4, x_2 x_5, x_2 x_6, x_3^2, x_3 x_4, x_3 x_5, x_3 x_6, x_4^2\}$

In[\*]:= **TM**

Out[\*]:=  $\{x_4 x_5^3, x_4 x_5^2 x_6, x_4 x_5 x_6^2, x_4 x_6^3, x_5^4, x_5^3 x_6, x_5^2 x_6^2, x_5 x_6^3, x_6^4\}$

In[\*]:= { **$\ell$** ,  **$\tau$** }

Out[\*]:= {16, 9}

In[\*]:=  **$\ell * \tau$**

Out[\*]:= 144

In[\*]:= { **$n$** ,  **$\mu$** }

Out[\*]:= {6, 28}

In[\*]:=  **$n * \mu$**

Out[\*]:= 168

In[\*]:= **findDimU[n, r, s,  $\delta$ , w,  $\ell$ ,  $\tau$ ]**

Out[\*]:= 186

Construct the border basis (**borBasis**) of a random distinguished ideal  $I$  of the given signature, and compute the dimension of the tangent space at  $[I] \in H$ .

We first compute the generators associated to the leading monomials, after which we append the non-leading boundary monomials.

In[\*]:= **borBasisA = Table[bdry[[j]] -  $\sum_{i=1}^{\tau}$  RandomInteger[{-1, 1}] \* TM[[i]], {j, 1,  $\ell$ }]**

Out[\*]:=  $\{x_1^2 - x_4 x_5^3 - x_5^4 - x_4 x_5^2 x_6 + x_4 x_5 x_6^2 + x_5^2 x_6^2 - x_5 x_6^3 - x_6^4,$   
 $x_1 x_2 + x_5^3 x_6 - x_5^2 x_6^2 - x_5 x_6^3, x_1 x_3 - x_5^4 - x_4 x_5^2 x_6 + x_5^3 x_6 - x_4 x_5 x_6^2 - x_5^2 x_6^2 + x_4 x_6^3 - x_5 x_6^3 + x_6^4,$   
 $x_1 x_4 + x_4 x_5^3 + x_5^4 - x_4 x_5^2 x_6 - x_5^3 x_6 - x_4 x_5 x_6^2 + x_5^2 x_6^2 + x_4 x_6^3 + x_5 x_6^3 - x_6^4,$   
 $x_1 x_5 + x_4 x_5^3 - x_4 x_5^2 x_6 - x_5^3 x_6 - x_4 x_5 x_6^2 + x_4 x_6^3 + x_5 x_6^3, -x_5^4 + x_1 x_6 + x_5^3 x_6 + x_5^2 x_6^2 - x_4 x_6^3,$   
 $x_2^2 + x_5^4 - x_5^3 x_6 - x_4 x_5 x_6^2 - x_5^2 x_6^2, x_2 x_3 + x_4 x_5^3 - x_5^4 + x_4 x_5^2 x_6 - x_5^3 x_6 - x_4 x_5 x_6^2 + x_5^2 x_6^2 + x_5 x_6^3 - x_6^4,$   
 $x_2 x_4 - x_4 x_5^3 + x_5^4 + x_4 x_5^2 x_6 - x_5^3 x_6 - x_4 x_5 x_6^2 + x_4 x_6^3 - x_5 x_6^3 + x_6^4,$   
 $x_2 x_5 - x_5^4 + x_4 x_5^2 x_6 + x_5^3 x_6 + x_4 x_5 x_6^2 + x_5^2 x_6^2, -x_4 x_5^3 - x_5^4 + x_2 x_6 - x_4 x_5^2 x_6 - x_5^3 x_6 + x_4 x_5 x_6^2 - x_5^2 x_6^2 - x_6^4,$   
 $x_3^2 + x_4 x_5^3 + x_5^4 + x_4 x_5^2 x_6 + x_5^2 x_6^2 - x_4 x_6^3 - x_5 x_6^3 + x_6^4, x_3 x_4 + x_4 x_5^3 - x_5^4 + x_4 x_5^2 x_6 - x_5^3 x_6 + x_5^2 x_6^2 + x_5 x_6^3,$   
 $x_3 x_5 + x_5^4 + x_4 x_5^2 x_6 - x_5^3 x_6 - x_4 x_5 x_6^2 - x_5^2 x_6^2 - x_4 x_6^3,$   
 $x_3 x_6 + x_4 x_5^2 x_6 - x_5^3 x_6 - x_5 x_6^3 + x_6^4, x_4^2 - x_4 x_5^3 + x_5^4 + x_4 x_5^2 x_6 - x_5^3 x_6 + x_5^2 x_6^2 + x_4 x_6^3 + x_6^4\}$

```
In[ ]:= borBasis = Join[borBasisA, Take[bdry, -(v - l)]]
```

```
Out[ ]:= {x1^2 - x4 x5^3 - x5^4 - x4 x5^2 x6 + x4 x5 x6^2 + x5^2 x6^2 - x5 x6^3 - x6^4,
  x1 x2 + x5^3 x6 - x5^2 x6^2 - x5 x6^3, x1 x3 - x5^4 - x4 x5^2 x6 + x5^3 x6 - x4 x5 x6^2 - x5^2 x6^2 + x4 x6^3 - x5 x6^3 + x6^4,
  x1 x4 + x4 x5^3 + x5^4 - x4 x5^2 x6 - x5^3 x6 - x4 x5 x6^2 + x5^2 x6^2 + x4 x6^3 + x5 x6^3 - x6^4,
  x1 x5 + x4 x5^3 - x4 x5^2 x6 - x5^3 x6 - x4 x5 x6^2 + x4 x6^3 + x5 x6^3, -x5^4 + x1 x6 + x5^3 x6 + x5^2 x6^2 - x4 x6^3,
  x2^2 + x5^4 - x5^3 x6 - x4 x5 x6^2 - x5^2 x6^2, x2 x3 + x4 x5^3 - x5^4 + x4 x5^2 x6 - x5^3 x6 - x4 x5 x6^2 + x5^2 x6^2 + x5 x6^3 - x6^4,
  x2 x4 - x4 x5^3 + x5^4 + x4 x5^2 x6 - x5^3 x6 - x4 x5 x6^2 + x4 x6^3 - x5 x6^3 + x6^4,
  x2 x5 - x5^4 + x4 x5^2 x6 + x5^3 x6 + x4 x5 x6^2 + x5^2 x6^2, -x4 x5^3 - x5^4 + x2 x6 - x4 x5^2 x6 - x5^3 x6 + x4 x5 x6^2 - x5^2 x6^2 - x6^4,
  x3^2 + x4 x5^3 + x5^4 + x4 x5^2 x6 + x5^2 x6^2 - x4 x6^3 - x5 x6^3 + x6^4, x3 x4 + x4 x5^3 - x5^4 + x4 x5^2 x6 - x5^3 x6 + x5^2 x6^2 + x5 x6^3,
  x3 x5 + x5^4 + x4 x5^2 x6 - x5^3 x6 - x4 x5 x6^2 - x5^2 x6^2 - x4 x6^3, x3 x6 + x4 x5^2 x6 - x5^3 x6 - x5 x6^3 + x6^4,
  x4^2 - x4 x5^3 + x5^4 + x4 x5^2 x6 - x5^3 x6 + x5^2 x6^2 + x4 x6^3 + x6^4, x1 x4 x5, x1 x4 x6, x1 x5^2, x1 x5 x6, x1 x6^2,
  x2 x4 x5, x2 x4 x6, x2 x5^2, x2 x5 x6, x2 x6^2, x3 x4 x5, x3 x4 x6, x3 x5^2, x3 x5 x6, x3 x6^2, x4 x5, x4 x6,
  x1 x4 x5^2, x1 x4 x5 x6, x1 x4 x6^2, x1 x5^3, x1 x5^2 x6, x1 x5 x6^2, x1 x6^3, x2 x4 x5^2, x2 x4 x5 x6, x2 x4 x6^2,
  x2 x5^3, x2 x5^2 x6, x2 x5 x6^2, x2 x6^3, x3 x4 x5^2, x3 x4 x5 x6, x3 x4 x6^2, x3 x5^3, x3 x5^2 x6, x3 x5 x6^2, x3 x6^3,
  x4 x5^2, x4 x5 x6, x4 x6^2, x1 x4 x5^3, x1 x4 x5^2 x6, x1 x4 x5 x6^2, x1 x4 x6^3, x1 x5^4, x1 x5^3 x6, x1 x5^2 x6^2,
  x1 x5 x6^3, x1 x6^4, x2 x4 x5^3, x2 x4 x5^2 x6, x2 x4 x5 x6^2, x2 x4 x6^3, x2 x5^4, x2 x5^3 x6, x2 x5^2 x6^2, x2 x5 x6^3,
  x2 x6^4, x3 x4 x5^3, x3 x4 x5^2 x6, x3 x4 x5 x6^2, x3 x4 x6^3, x3 x5^4, x3 x5^3 x6, x3 x5^2 x6^2, x3 x5 x6^3, x3 x6^4, x4 x5^3,
  x4 x5^2 x6, x4 x5 x6^2, x4 x6^3, x4 x5^4, x4 x5^3 x6, x4 x5^2 x6^2, x4 x5 x6^3, x4 x6^4, x5^5, x5^4 x6, x5^3 x6^2, x5^2 x6^3, x5 x6^4, x6^5}
```

Find the tangent space relations and the dimension of the tangent space at [I]

```
In[ ]:= {aLst, allTanSpaceReIns} = makeTanSpaceReIns[borBasis, basis, bdry, varList];
```

```
In[ ]:= aLstLength = Length[aLst]
```

```
Out[ ]:= 2772
```

```
In[ ]:= tanSpaceDim[Length[aLst], allTanSpaceReIns]
```

```
Out[ ]:= 186
```

```
In[ ]:= findDimU[n, r, s, δ, w, l, τ]
```

```
Out[ ]:= 186
```

Since  $\dim(U) = 186$ , this shows that [I] is a smooth point on an elementary component of dimension 186.

The dimension of the principal component is:

```
In[ ]:= μ * n
```

```
Out[ ]:= 168
```
