# Supplementary material for: More elementary components of the Hilbert scheme of points
Source: arXiv:2102.00494 ancillary file (2022-08-29)
Supplement: Supplementary file 8 [file signature_6,3,4,3,2.pdf]

# Signature (6, 3, 4, 3, 2)

In this case, sufficiently general distinguished ideals of this signature (and Hilbert function (1, 6, 21, 10, 15) are smooth points on an elementary component of dimension 705. The principal component has dimension  $6 \cdot 53 = 318$ .

**Note:** To execute this file, the notebook titled *utility functions for paper.nb* must be executed first.

---

## Set up the example.

```
In[ ]:= n = 6;  
varList = Table[xi, {i, 1, n}]
```

```
Out[ ]:= {x1, x2, x3, x4, x5, x6}
```

The next function **makeBasisAndBoundaryMonomialLists** computes and returns the lists of basis and boundary monomials, the Hilbert function, the leading monomials LM, the trailing monomials TM, the sets  $\mathcal{T}' = \text{TarPrime}$  and  $\mathcal{T} = \text{Tar}$ , and the parameters

$\mu = |\text{basis}|$ ,  $\nu = |\text{bdry}|$ ,  $\ell = |\text{LM}|$ , and  $\tau = |\text{TM}|$ . This function is defined in the notebook *Utilities for modification construction 2020.nb*.

```
In[ ]:= {basis, bdry, H, LM, TM, tarPrime, tar,  $\mu$ ,  $\nu$ ,  $\ell$ ,  $\tau$ } =  
makeBasisAndBoundaryMonomialLists[n, r = 3, s = 4,  $\delta$  = 3, w = 2];
```

```
In[ ]:= basis
```

```
Out[ ]:= {1, x1, x2, x3, x4, x5, x6, x12, x1 x2, x1 x3, x1 x4, x1 x5, x1 x6, x22, x2 x3, x2 x4, x2 x5, x2 x6, x32, x3 x4,  
x3 x5, x3 x6, x42, x4 x5, x4 x6, x52, x5 x6, x62, x43, x42 x5, x42 x6, x4 x52, x4 x5 x6, x4 x62, x53, x52 x6, x5 x62,  
x63, x44, x43 x5, x43 x6, x42 x52, x42 x5 x6, x42 x62, x4 x53, x4 x52 x6, x4 x5 x62, x4 x63, x54, x53 x6, x52 x62, x5 x63, x64}
```

```
In[ ]:=  $\mu$ 
```

```
Out[ ]:= 53
```

In[\*]:= **bdry**

Out[\*]=  $\{x_1^3, x_1^2 x_2, x_1^2 x_3, x_1^2 x_4, x_1^2 x_5, x_1^2 x_6, x_1 x_2^2, x_1 x_2 x_3, x_1 x_2 x_4, x_1 x_2 x_5, x_1 x_2 x_6, x_1 x_3^2, x_1 x_3 x_4, x_1 x_3 x_5, x_1 x_3 x_6, x_1 x_4^2, x_1 x_4 x_5, x_1 x_4 x_6, x_1 x_5^2, x_1 x_5 x_6, x_1 x_6^2, x_2^3, x_2^2 x_3, x_2^2 x_4, x_2^2 x_5, x_2^2 x_6, x_2 x_3^2, x_2 x_3 x_4, x_2 x_3 x_5, x_2 x_3 x_6, x_2 x_4^2, x_2 x_4 x_5, x_2 x_4 x_6, x_2 x_5^2, x_2 x_5 x_6, x_2 x_6^2, x_3^3, x_3^2 x_4, x_3^2 x_5, x_3^2 x_6, x_3 x_4^2, x_3 x_4 x_5, x_3 x_4 x_6, x_3 x_5^2, x_3 x_5 x_6, x_3 x_6^2, x_4^3, x_4^2 x_5, x_4^2 x_6, x_4 x_5^3, x_4 x_5^2 x_6, x_4 x_6^2, x_5^3, x_5^2 x_6, x_5 x_6^2, x_6^3, x_6^2 x_5, x_6 x_5^2, x_6 x_4^2, x_6 x_4 x_5, x_6 x_4 x_6, x_6 x_5^2, x_6 x_5 x_6, x_6 x_6^2, x_7^3, x_7^2 x_8, x_7^2 x_9, x_7^2 x_{10}, x_7^2 x_{11}, x_7^2 x_{12}, x_7 x_8^2, x_7 x_8 x_9, x_7 x_8 x_{10}, x_7 x_8 x_{11}, x_7 x_8 x_{12}, x_7 x_9^2, x_7 x_9 x_{10}, x_7 x_9 x_{11}, x_7 x_9 x_{12}, x_7 x_{10}^2, x_7 x_{10} x_{11}, x_7 x_{10} x_{12}, x_7 x_{11}^2, x_7 x_{11} x_{12}, x_7 x_{12}^2, x_8^3, x_8^2 x_9, x_8^2 x_{10}, x_8^2 x_{11}, x_8^2 x_{12}, x_8 x_9^2, x_8 x_9 x_{10}, x_8 x_9 x_{11}, x_8 x_9 x_{12}, x_8 x_{10}^2, x_8 x_{10} x_{11}, x_8 x_{10} x_{12}, x_8 x_{11}^2, x_8 x_{11} x_{12}, x_8 x_{12}^2, x_9^3, x_9^2 x_{10}, x_9^2 x_{11}, x_9^2 x_{12}, x_9 x_{10}^2, x_9 x_{10} x_{11}, x_9 x_{10} x_{12}, x_9 x_{11}^2, x_9 x_{11} x_{12}, x_9 x_{12}^2, x_{10}^3, x_{10}^2 x_{11}, x_{10}^2 x_{12}, x_{10} x_{11}^2, x_{10} x_{11} x_{12}, x_{10} x_{12}^2, x_{11}^3, x_{11}^2 x_{12}, x_{11} x_{12}^2, x_{12}^3, x_{12}^2 x_{11}, x_{12} x_{11}^2, x_{12} x_{11} x_{12}, x_{13}^3, x_{13}^2 x_{14}, x_{13}^2 x_{15}, x_{13}^2 x_{16}, x_{13} x_{14}^2, x_{13} x_{14} x_{15}, x_{13} x_{14} x_{16}, x_{13} x_{15}^2, x_{13} x_{15} x_{16}, x_{13} x_{16}^2, x_{14}^3, x_{14}^2 x_{15}, x_{14}^2 x_{16}, x_{14} x_{15}^2, x_{14} x_{15} x_{16}, x_{14} x_{16}^2, x_{15}^3, x_{15}^2 x_{16}, x_{15} x_{16}^2, x_{16}^3, x_{16}^2 x_{15}, x_{16} x_{15}^2, x_{16} x_{15} x_{16}, x_{17}^3, x_{17}^2 x_{18}, x_{17}^2 x_{19}, x_{17}^2 x_{20}, x_{17}^2 x_{21}, x_{17}^2 x_{22}, x_{17} x_{18}^2, x_{17} x_{18} x_{19}, x_{17} x_{18} x_{20}, x_{17} x_{18} x_{21}, x_{17} x_{18} x_{22}, x_{17} x_{19}^2, x_{17} x_{19} x_{20}, x_{17} x_{19} x_{21}, x_{17} x_{19} x_{22}, x_{17} x_{20}^2, x_{17} x_{20} x_{21}, x_{17} x_{20} x_{22}, x_{17} x_{21}^2, x_{17} x_{21} x_{22}, x_{17} x_{22}^2, x_{18}^3, x_{18}^2 x_{19}, x_{18}^2 x_{20}, x_{18}^2 x_{21}, x_{18}^2 x_{22}, x_{18} x_{19}^2, x_{18} x_{19} x_{20}, x_{18} x_{19} x_{21}, x_{18} x_{19} x_{22}, x_{18} x_{20}^2, x_{18} x_{20} x_{21}, x_{18} x_{20} x_{22}, x_{18} x_{21}^2, x_{18} x_{21} x_{22}, x_{18} x_{22}^2, x_{19}^3, x_{19}^2 x_{20}, x_{19}^2 x_{21}, x_{19}^2 x_{22}, x_{19} x_{20}^2, x_{19} x_{20} x_{21}, x_{19} x_{20} x_{22}, x_{19} x_{21}^2, x_{19} x_{21} x_{22}, x_{19} x_{22}^2, x_{20}^3, x_{20}^2 x_{21}, x_{20}^2 x_{22}, x_{20} x_{21}^2, x_{20} x_{21} x_{22}, x_{20} x_{22}^2, x_{21}^3, x_{21}^2 x_{20}, x_{21}^2 x_{22}, x_{21} x_{20}^2, x_{21} x_{20} x_{22}, x_{21} x_{22}^2, x_{22}^3, x_{22}^2 x_{21}, x_{22} x_{21}^2, x_{22} x_{21} x_{22}, x_{23}^3, x_{23}^2 x_{24}, x_{23}^2 x_{25}, x_{23}^2 x_{26}, x_{23} x_{24}^2, x_{23} x_{24} x_{25}, x_{23} x_{24} x_{26}, x_{23} x_{25}^2, x_{23} x_{25} x_{26}, x_{23} x_{26}^2, x_{24}^3, x_{24}^2 x_{25}, x_{24}^2 x_{26}, x_{24} x_{25}^2, x_{24} x_{25} x_{26}, x_{24} x_{26}^2, x_{25}^3, x_{25}^2 x_{26}, x_{25} x_{26}^2, x_{26}^3, x_{26}^2 x_{25}, x_{26} x_{25}^2, x_{26} x_{25} x_{26}, x_{27}^3, x_{27}^2 x_{28}, x_{27}^2 x_{29}, x_{27}^2 x_{30}, x_{27}^2 x_{31}, x_{27}^2 x_{32}, x_{27} x_{28}^2, x_{27} x_{28} x_{29}, x_{27} x_{28} x_{30}, x_{27} x_{28} x_{31}, x_{27} x_{28} x_{32}, x_{27} x_{29}^2, x_{27} x_{29} x_{30}, x_{27} x_{29} x_{31}, x_{27} x_{29} x_{32}, x_{27} x_{30}^2, x_{27} x_{30} x_{31}, x_{27} x_{30} x_{32}, x_{27} x_{31}^2, x_{27} x_{31} x_{32}, x_{27} x_{32}^2, x_{28}^3, x_{28}^2 x_{29}, x_{28}^2 x_{30}, x_{28}^2 x_{31}, x_{28}^2 x_{32}, x_{28} x_{29}^2, x_{28} x_{29} x_{30}, x_{28} x_{29} x_{31}, x_{28} x_{29} x_{32}, x_{28} x_{30}^2, x_{28} x_{30} x_{31}, x_{28} x_{30} x_{32}, x_{28} x_{31}^2, x_{28} x_{31} x_{32}, x_{28} x_{32}^2, x_{29}^3, x_{29}^2 x_{30}, x_{29}^2 x_{31}, x_{29}^2 x_{32}, x_{29} x_{30}^2, x_{29} x_{30} x_{31}, x_{29} x_{30} x_{32}, x_{29} x_{31}^2, x_{29} x_{31} x_{32}, x_{29} x_{32}^2, x_{30}^3, x_{30}^2 x_{31}, x_{30}^2 x_{32}, x_{30} x_{31}^2, x_{30} x_{31} x_{32}, x_{30} x_{32}^2, x_{31}^3, x_{31}^2 x_{30}, x_{31}^2 x_{32}, x_{31} x_{30}^2, x_{31} x_{30} x_{32}, x_{31} x_{32}^2, x_{32}^3, x_{32}^2 x_{31}, x_{32} x_{31}^2, x_{32} x_{31} x_{32}, x_{33}^3, x_{33}^2 x_{34}, x_{33}^2 x_{35}, x_{33}^2 x_{36}, x_{33} x_{34}^2, x_{33} x_{34} x_{35}, x_{33} x_{34} x_{36}, x_{33} x_{35}^2, x_{33} x_{35} x_{36}, x_{33} x_{36}^2, x_{34}^3, x_{34}^2 x_{35}, x_{34}^2 x_{36}, x_{34} x_{35}^2, x_{34} x_{35} x_{36}, x_{34} x_{36}^2, x_{35}^3, x_{35}^2 x_{36}, x_{35} x_{36}^2, x_{36}^3, x_{36}^2 x_{35}, x_{36} x_{35}^2, x_{36} x_{35} x_{36}, x_{37}^3, x_{37}^2 x_{38}, x_{37}^2 x_{39}, x_{37}^2 x_{40}, x_{37}^2 x_{41}, x_{37}^2 x_{42}, x_{37} x_{38}^2, x_{37} x_{38} x_{39}, x_{37} x_{38} x_{40}, x_{37} x_{38} x_{41}, x_{37} x_{38} x_{42}, x_{37} x_{39}^2, x_{37} x_{39} x_{40}, x_{37} x_{39} x_{41}, x_{37} x_{39} x_{42}, x_{37} x_{40}^2, x_{37} x_{40} x_{41}, x_{37} x_{40} x_{42}, x_{37} x_{41}^2, x_{37} x_{41} x_{42}, x_{37} x_{42}^2, x_{38}^3, x_{38}^2 x_{39}, x_{38}^2 x_{40}, x_{38}^2 x_{41}, x_{38}^2 x_{42}, x_{38} x_{39}^2, x_{38} x_{39} x_{40}, x_{38} x_{39} x_{41}, x_{38} x_{39} x_{42}, x_{38} x_{40}^2, x_{38} x_{40} x_{41}, x_{38} x_{40} x_{42}, x_{38} x_{41}^2, x_{38} x_{41} x_{42}, x_{38} x_{42}^2, x_{39}^3, x_{39}^2 x_{40}, x_{39}^2 x_{41}, x_{39}^2 x_{42}, x_{39} x_{40}^2, x_{39} x_{40} x_{41}, x_{39} x_{40} x_{42}, x_{39} x_{41}^2, x_{39} x_{41} x_{42}, x_{39} x_{42}^2, x_{40}^3, x_{40}^2 x_{41}, x_{40}^2 x_{42}, x_{40} x_{41}^2, x_{40} x_{41} x_{42}, x_{40} x_{42}^2, x_{41}^3, x_{41}^2 x_{40}, x_{41}^2 x_{42}, x_{41} x_{40}^2, x_{41} x_{40} x_{42}, x_{41} x_{42}^2, x_{42}^3, x_{42}^2 x_{41}, x_{42} x_{41}^2, x_{42} x_{41} x_{42}, x_{43}^3, x_{43}^2 x_{44}, x_{43}^2 x_{45}, x_{43}^2 x_{46}, x_{43} x_{44}^2, x_{43} x_{44} x_{45}, x_{43} x_{44} x_{46}, x_{43} x_{45}^2, x_{43} x_{45} x_{46}, x_{43} x_{46}^2, x_{44}^3, x_{44}^2 x_{45}, x_{44}^2 x_{46}, x_{44} x_{45}^2, x_{44} x_{45} x_{46}, x_{44} x_{46}^2, x_{45}^3, x_{45}^2 x_{46}, x_{45} x_{46}^2, x_{46}^3, x_{46}^2 x_{45}, x_{46} x_{45}^2, x_{46} x_{45} x_{46}, x_{47}^3, x_{47}^2 x_{48}, x_{47}^2 x_{49}, x_{47}^2 x_{50}, x_{47}^2 x_{51}, x_{47}^2 x_{52}, x_{47} x_{48}^2, x_{47} x_{48} x_{49}, x_{47} x_{48} x_{50}, x_{47} x_{48} x_{51}, x_{47} x_{48} x_{52}, x_{47} x_{49}^2, x_{47} x_{49} x_{50}, x_{47} x_{49} x_{51}, x_{47} x_{49} x_{52}, x_{47} x_{50}^2, x_{47} x_{50} x_{51}, x_{47} x_{50} x_{52}, x_{47} x_{51}^2, x_{47} x_{51} x_{52}, x_{47} x_{52}^2, x_{48}^3, x_{48}^2 x_{49}, x_{48}^2 x_{50}, x_{48}^2 x_{51}, x_{48}^2 x_{52}, x_{48} x_{49}^2, x_{48} x_{49} x_{50}, x_{48} x_{49} x_{51}, x_{48} x_{49} x_{52}, x_{48} x_{50}^2, x_{48} x_{50} x_{51}, x_{48} x_{50} x_{52}, x_{48} x_{51}^2, x_{48} x_{51} x_{52}, x_{48} x_{52}^2, x_{49}^3, x_{49}^2 x_{50}, x_{49}^2 x_{51}, x_{49}^2 x_{52}, x_{49} x_{50}^2, x_{49} x_{50} x_{51}, x_{49} x_{50} x_{52}, x_{49} x_{51}^2, x_{49} x_{51} x_{52}, x_{49} x_{52}^2, x_{50}^3, x_{50}^2 x_{51}, x_{50}^2 x_{52}, x_{50} x_{51}^2, x_{50} x_{51} x_{52}, x_{50} x_{52}^2, x_{51}^3, x_{51}^2 x_{50}, x_{51}^2 x_{52}, x_{51} x_{50}^2, x_{51} x_{50} x_{52}, x_{51} x_{52}^2, x_{52}^3, x_{52}^2 x_{51}, x_{52} x_{51}^2, x_{52} x_{51} x_{52}, x_{53}^3, x_{53}^2 x_{54}, x_{53}^2 x_{55}, x_{53}^2 x_{56}, x_{53} x_{54}^2, x_{53} x_{54} x_{55}, x_{53} x_{54} x_{56}, x_{53} x_{55}^2, x_{53} x_{55} x_{56}, x_{53} x_{56}^2, x_{54}^3, x_{54}^2 x_{55}, x_{54}^2 x_{56}, x_{54} x_{55}^2, x_{54} x_{55} x_{56}, x_{54} x_{56}^2, x_{55}^3, x_{55}^2 x_{56}, x_{55} x_{56}^2, x_{56}^3, x_{56}^2 x_{55}, x_{56} x_{55}^2, x_{56} x_{55} x_{56}, x_{57}^3, x_{57}^2 x_{58}, x_{57}^2 x_{59}, x_{57}^2 x_{60}, x_{57}^2 x_{61}, x_{57}^2 x_{62}, x_{57} x_{58}^2, x_{57} x_{58} x_{59}, x_{57} x_{58} x_{60}, x_{57} x_{58} x_{61}, x_{57} x_{58} x_{62}, x_{57} x_{59}^2, x_{57} x_{59} x_{60}, x_{57} x_{59} x_{61}, x_{57} x_{59} x_{62}, x_{57} x_{60}^2, x_{57} x_{60} x_{61}, x_{57} x_{60} x_{62}, x_{57} x_{61}^2, x_{57} x_{61} x_{62}, x_{57} x_{62}^2, x_{58}^3, x_{58}^2 x_{59}, x_{58}^2 x_{60}, x_{58}^2 x_{61}, x_{58}^2 x_{62}, x_{58} x_{59}^2, x_{58} x_{59} x_{60}, x_{58} x_{59} x_{61}, x_{58} x_{59} x_{62}, x_{58} x_{60}^2, x_{58} x_{60} x_{61}, x_{58} x_{60} x_{62}, x_{58} x_{61}^2, x_{58} x_{61} x_{62}, x_{58} x_{62}^2, x_{59}^3, x_{59}^2 x_{60}, x_{59}^2 x_{61}, x_{59}^2 x_{62}, x_{59} x_{60}^2, x_{59} x_{60} x_{61}, x_{59} x_{60} x_{62}, x_{59} x_{61}^2, x_{59} x_{61} x_{62}, x_{59} x_{62}^2, x_{60}^3, x_{60}^2 x_{61}, x_{60}^2 x_{62}, x_{60} x_{61}^2, x_{60} x_{61} x_{62}, x_{60} x_{62}^2, x_{61}^3, x_{61}^2 x_{60}, x_{61}^2 x_{62}, x_{61} x_{60}^2, x_{61} x_{60} x_{62}, x_{61} x_{62}^2, x_{62}^3, x_{62}^2 x_{61}, x_{62} x_{61}^2, x_{62} x_{61} x_{62}, x_{63}^3, x_{63}^2 x_{64}, x_{63}^2 x_{65}, x_{63}^2 x_{66}, x_{63} x_{64}^2, x_{63} x_{64} x_{65}, x_{63} x_{64} x_{66}, x_{63} x_{65}^2, x_{63} x_{65} x_{66}, x_{63} x_{66}^2, x_{64}^3, x_{64}^2 x_{65}, x_{64}^2 x_{66}, x_{64} x_{65}^2, x_{64} x_{65} x_{66}, x_{64} x_{66}^2, x_{65}^3, x_{65}^2 x_{66}, x_{65} x_{66}^2, x_{66}^3, x_{66}^2 x_{65}, x_{66} x_{65}^2, x_{66} x_{65} x_{66}, x_{67}^3, x_{67}^2 x_{68}, x_{67}^2 x_{69}, x_{67}^2 x_{70}, x_{67}^2 x_{71}, x_{67}^2 x_{72}, x_{67} x_{68}^2, x_{67} x_{68} x_{69}, x_{67} x_{68} x_{70}, x_{67} x_{68} x_{71}, x_{67} x_{68} x_{72}, x_{67} x_{69}^2, x_{67} x_{69} x_{70}, x_{67} x_{69} x_{71}, x_{67} x_{69} x_{72}, x_{67} x_{70}^2, x_{67} x_{70} x_{71}, x_{67} x_{70} x_{72}, x_{67} x_{71}^2, x_{67} x_{71} x_{72}, x_{67} x_{72}^2, x_{68}^3, x_{68}^2 x_{69}, x_{68}^2 x_{70}, x_{68}^2 x_{71}, x_{68}^2 x_{72}, x_{68} x_{69}^2, x_{68} x_{69} x_{70}, x_{68} x_{69} x_{71}, x_{68} x_{69} x_{72}, x_{68} x_{70}^2, x_{68} x_{70} x_{71}, x_{68} x_{70} x_{72}, x_{68} x_{71}^2, x_{68} x_{71} x_{72}, x_{68} x_{72}^2, x_{69}^3, x_{69}^2 x_{70}, x_{69}^2 x_{71}, x_{69}^2 x_{72}, x_{69} x_{70}^2, x_{69} x_{70} x_{71}, x_{69} x_{70} x_{72}, x_{69} x_{71}^2, x_{69} x_{71} x_{72}, x_{69} x_{72}^2, x_{70}^3, x_{70}^2 x_{71}, x_{70}^2 x_{72}, x_{70} x_{71}^2, x_{70} x_{71} x_{72}, x_{70} x_{72}^2, x_{71}^3, x_{71}^2 x_{70}, x_{71}^2 x_{72}, x_{71} x_{70}^2, x_{71} x_{70} x_{72}, x_{71} x_{72}^2, x_{72}^3, x_{72}^2 x_{71}, x_{72} x_{71}^2, x_{72} x_{71} x_{72}, x_{73}^3, x_{73}^2 x_{74}, x_{73}^2 x_{75}, x_{73}^2 x_{76}, x_{73} x_{74}^2, x_{73} x_{74} x_{75}, x_{73} x_{74} x_{76}, x_{73} x_{75}^2, x_{73} x_{75} x_{76}, x_{73} x_{76}^2, x_{74}^3, x_{74}^2 x_{75}, x_{74}^2 x_{76}, x_{74} x_{75}^2, x_{74} x_{75} x_{76}, x_{74} x_{76}^2, x_{75}^3, x_{75}^2 x_{76}, x_{75} x_{76}^2, x_{76}^3, x_{76}^2 x_{75}, x_{76} x_{75}^2, x_{76} x_{75} x_{76}, x_{77}^3, x_{77}^2 x_{78}, x_{77}^2 x_{79}, x_{77}^2 x_{80}, x_{77}^2 x_{81}, x_{77}^2 x_{82}, x_{77} x_{78}^2, x_{77} x_{78} x_{79}, x_{77} x_{78} x_{80}, x_{77} x_{78} x_{81}, x_{77} x_{78} x_{82}, x_{77} x_{79}^2, x_{77} x_{79} x_{80}, x_{77} x_{79} x_{81}, x_{77} x_{79} x_{82}, x_{77} x_{80}^2, x_{77} x_{80} x_{81}, x_{77} x_{80} x_{82}, x_{77} x_{81}^2, x_{77} x_{81} x_{82}, x_{77} x_{82}^2, x_{78}^3, x_{78}^2 x_{79}, x_{78}^2 x_{80}, x_{78}^2 x_{81}, x_{78}^2 x_{82}, x_{78} x_{79}^2, x_{78} x_{79} x_{80}, x_{78} x_{79} x_{81}, x_{78} x_{79} x_{82}, x_{78} x_{80}^2, x_{78} x_{80} x_{81}, x_{78} x_{80} x_{82}, x_{78} x_{81}^2, x_{78} x_{81} x_{82}, x_{78} x_{82}^2, x_{79}^3, x_{79}^2 x_{80}, x_{79}^2 x_{81}, x_{79}^2 x_{82}, x_{79} x_{80}^2, x_{79} x_{80} x_{81}, x_{79} x_{80} x_{82}, x_{79} x_{81}^2, x_{79} x_{81} x_{82}, x_{79} x_{82}^2, x_{80}^3, x_{80}^2 x_{81}, x_{80}^2 x_{82}, x_{80} x_{81}^2, x_{80} x_{81} x_{82}, x_{80} x_{82}^2, x_{81}^3, x_{81}^2 x_{80}, x_{81}^2 x_{82}, x_{81} x_{80}^2, x_{81} x_{80} x_{82}, x_{81} x_{82}^2, x_{82}^3, x_{82}^2 x_{81}, x_{82} x_{81}^2, x_{82} x_{81} x_{82}, x_{83}^3, x_{83}^2 x_{84}, x_{83}^2 x_{85}, x_{83}^2 x_{86}, x_{83} x_{84}^2, x_{83} x_{84} x_{85}, x_{83} x_{84} x_{86}, x_{83} x_{85}^2, x_{83} x_{85} x_{86}, x_{83} x_{86}^2, x_{84}^3, x_{84}^2 x_{85}, x_{84}^2 x_{86}, x_{84} x_{85}^2, x_{84} x_{85} x_{86}, x_{84} x_{86}^2, x_{85}^3, x_{85}^2 x_{86}, x_{85} x_{86}^2, x_{86}^3, x_{86}^2 x_{85}, x_{86} x_{85}^2, x_{86} x_{85} x_{86}, x_{87}^3, x_{87}^2 x_{88}, x_{87}^2 x_{89}, x_{87}^2 x_{90}, x_{87}^2 x_{91}, x_{87}^2 x_{92}, x_{87} x_{88}^2, x_{87} x_{88} x_{89}, x_{87} x_{88} x_{90}, x_{87} x_{88} x_{91}, x_{87} x_{88} x_{92}, x_{87} x_{89}^2, x_{87} x_{89} x_{90}, x_{87} x_{89} x_{91}, x_{87} x_{89} x_{92}, x_{87} x_{90}^2, x_{87} x_{90} x_{91}, x_{87} x_{90} x_{92}, x_{87} x_{91}^2, x_{87} x_{91} x_{92}, x_{87} x_{92}^2, x_{88}^3, x_{88}^2 x_{89}, x_{88}^2 x_{90}, x_{88}^2 x_{91}, x_{88}^2 x_{92}, x_{88} x_{89}^2, x_{88} x_{89} x_{90}, x_{88} x_{89} x_{91}, x_{88} x_{89} x_{92}, x_{88} x_{90}^2, x_{88} x_{90} x_{91}, x_{88} x_{90} x_{92}, x_{88} x_{91}^2, x_{88} x_{91} x_{92}, x_{88} x_{92}^2, x_{89}^3, x_{89}^2 x_{90}, x_{89}^2 x_{91}, x_{89}^2 x_{92}, x_{89} x_{90}^2, x_{89} x_{90} x_{91}, x_{89} x_{90} x_{92}, x_{89} x_{91}^2, x_{89} x_{91} x_{92}, x_{89} x_{92}^2, x_{90}^3, x_{90}^2 x_{91}, x_{90}^2 x_{92}, x_{90} x_{91}^2, x_{90} x_{91} x_{92}, x_{90} x_{92}^2, x_{91}^3, x_{91}^2 x_{90}, x_{91}^2 x_{92}, x_{91} x_{90}^2, x_{91} x_{90} x_{92}, x_{91} x_{92}^2, x_{92}^3, x_{92}^2 x_{91}, x_{92} x_{91}^2, x_{92} x_{91} x_{92}, x_{93}^3, x_{93}^2 x_{94}, x_{93}^2 x_{95}, x_{93}^2 x_{96}, x_{93} x_{94}^2, x_{93} x_{94} x_{95}, x_{93} x_{94} x_{96}, x_{93} x_{95}^2, x_{93} x_{95} x_{96}, x_{93} x_{96}^2, x_{94}^3, x_{94}^2 x_{95}, x_{94}^2 x_{96}, x_{94} x_{95}^2, x_{94} x_{95} x_{96}, x_{94} x_{96}^2, x_{95}^3, x_{95}^2 x_{96}, x_{95} x_{96}^2, x_{96}^3, x_{96}^2 x_{95}, x_{96} x_{95}^2, x_{96} x_{95} x_{96}, x_{97}^3, x_{97}^2 x_{98}, x_{97}^2 x_{99}, x_{97}^2 x_{100}, x_{97}^2 x_{101}, x_{97}^2 x_{102}, x_{97} x_{98}^2, x_{97} x_{98} x_{99}, x_{97} x_{98} x_{100}, x_{97} x_{98} x_{101}, x_{97} x_{98} x_{102}, x_{97} x_{99}^2, x_{97} x_{99} x_{100}, x_{97} x_{99} x_{101}, x_{97} x_{99} x_{102}, x_{97} x_{100}^2, x_{97} x_{100} x_{101}, x_{97} x_{100} x_{102}, x_{97} x_{101}^2, x_{97} x_{101} x_{102}, x_{97} x_{102}^2, x_{98}^3, x_{98}^2 x_{99}, x_{98}^2 x_{100}, x_{98}^2 x_{101}, x_{98}^2 x_{102}, x_{98} x_{99}^2, x_{98} x_{99} x_{100}, x_{98} x_{99} x_{101}, x_{98} x_{99} x_{102}, x_{98} x_{100}^2, x_{98} x_{100} x_{101}, x_{98} x_{100} x_{102}, x_{98} x_{101}^2, x_{98} x_{101} x_{102}, x_{98} x_{102}^2, x_{99}^3, x_{99}^2 x_{100}, x_{99}^2 x_{101}, x_{99}^2 x_{102}, x_{99} x_{100}^2, x_{99} x_{100} x_{101}, x_{99} x_{100} x_{102}, x_{99} x_{101}^2, x_{99} x_{101} x_{102}, x_{99} x_{102}^2, x_{100}^3, x_{100}^2 x_{101}, x_{100}^2 x_{102}, x_{100} x_{101}^2, x_{100} x_{101} x_{102}, x_{100} x_{102}^2, x_{101}^3, x_{101}^2 x_{100}, x_{101}^2 x_{102}, x_{101} x_{100}^2, x_{101} x_{100} x_{102}, x_{101} x_{102}^2, x_{102}^3, x_{102}^2 x_{101}, x_{102} x_{101}^2, x_{102} x_{101} x_{102}, x_{103}^3, x_{103}^2 x_{104}, x_{103}^2 x_{105}, x_{103}^2 x_{106}, x_{103} x_{104}^2, x_{103} x_{104} x_{105}, x_{103} x_{104} x_{106}, x_{103} x_{105}^2, x_{103} x_{105} x_{106}, x_{103} x_{106}^2, x_{104}^3, x_{104}^2 x_{105}, x_{104}^2 x_{106}, x_{104} x_{105}^2, x_{104} x_{105} x_{106}, x_{104} x_{106}^2, x_{105}^3, x_{105}^2 x_{106}, x_{105} x_{106}^2, x_{106}^3, x_{106}^2 x_{105}, x_{106} x_{105}^2, x_{106} x_{105} x_{106}, x_{107}^3, x_{107}^2 x_{108}, x_{107}^2 x_{109}, x_{107}^2 x_{110}, x_{107}^2 x_{111}, x_{107}^2 x_{112}, x_{107} x_{108}^2, x_{107} x_{108} x_{109}, x_{107} x_{108} x_{110}, x_{107} x_{108} x_{111}, x_{107} x_{108} x_{112}, x_{107} x_{109}^2, x_{107} x_{109} x_{110}, x_{107} x_{109} x_{111}, x_{107} x_{109} x_{112}, x_{107} x_{110}^2, x_{107} x_{110} x_{111}, x_{107} x_{110} x_{112}, x_{107} x_{111}^2, x_{107} x_{111} x_{112}, x_{107} x_{112}^2, x_{108}^3, x_{108}^2 x_{109}, x_{108}^2 x_{110}, x_{108}^2 x_{111}, x_{108}^2 x_{112}, x_{108} x_{109}^2, x_{108} x_{109} x_{110}, x_{108} x_{109} x_{111}, x_{108} x_{109} x_{112}, x_{108} x_{110}^2, x_{108} x_{110} x_{111}, x_{108} x_{110} x_{112}, x_{108} x_{111}^2, x_{108} x_{111} x_{112}, x_{108} x_{112}^2, x_{109}^3, x_{109}^2 x_{110}, x_{109}^2 x_{111}, x_{109}^2 x_{112}, x_{109} x_{110}^2, x_{109} x_{110} x_{111}, x_{109} x_{110} x_{112}, x_{109} x_{111}^2, x_{109} x_{111} x_{112}, x_{109} x_{112}^2, x_{110}^3, x_{110}^2 x_{111}, x_{110}^2 x_{112}, x_{110} x_{111}^2, x_{110} x_{111} x_{112}, x_{110} x_{112}^2, x_{111}^3, x_{111}^2 x_{110}, x_{111}^2 x_{112}, x_{111} x_{110}^2, x_{111} x_{1$

Construct the border basis (**borBasis**) of a random distinguished ideal  $I$  of the given signature, and compute the dimension of the tangent space at  $[I] \in H$ .

We first compute the generators associated to the leading monomials, after which we append the non-leading boundary monomials.

```
In[ ]:= borBasisA = Table[bdry[[j]] -  $\sum_{i=1}^{\tau}$  RandomInteger[{-1, 1}] * TM[[i]], {j, 1,  $\ell$ }] ;
In[ ]:= borBasis = Join[borBasisA, Take[bdry, - (v -  $\ell$ )]] ;
```

Find the tangent space relations and the dimension of the tangent space at  $[I]$

```
In[ ]:= {aLst, allTanSpaceReIns} = makeTanSpaceReIns[borBasis, basis, bdry, varList] ;
In[ ]:= aLstLength = Length[aLst]
Out[ ]:= 7526

In[ ]:= modulus = Prime[1000] ;
In[ ]:= tanSpaceDim[aLstLength, allTanSpaceReIns, modulus]
Out[ ]:= 705
```

Since  $\dim(U) = 705$ , this shows that  $[I]$  is a smooth point on an elementary component of dimension 705.

```
In[ ]:=
```

The dimension of the principal component is:

```
In[ ]:=  $\mu * n$ 
Out[ ]:= 318

In[ ]:=

In[ ]:=
```
