# Supplementary material for: More elementary components of the Hilbert scheme of points
Source: arXiv:2102.00494 ancillary file (2022-08-29)
Supplement: Supplementary file 10 [file utility_functions_for_paper.pdf]

# Utility functions for paper titled *More elementary components of the Hilbert scheme of points*

---

## I. Basic utility functions

Assign the number of variables and construct a list of the variables  $x_i$  and a list of “null substitutions”  $x_i \rightarrow 0$ .

```
In[ ]:= n = 3;  
varList = Table[xi, {i, 1, n}]
```

```
Out[ ]:= {x1, x2, x3}
```

```
In[ ]:= makeNullSubLst[itemList_] := Table[itemList[[i]] → 0, {i, 1, Length[itemList]}];  
nullSubs = makeNullSubLst[varList]
```

```
Out[ ]:= {x1 → 0, x2 → 0, x3 → 0}
```

The following function returns a list of the monomials of the given degree  $\text{deg}$  in the variables  $x_{\min\text{Var}} \dots x_{\max\text{Var}}$ . The list is in decreasing lex order ( $x_1 > x_2 > \dots > x_n$ ).

```
In[ ]:= allDegMonoms[deg_, maxVar_, minVar_] := Module[{result, i},
  (
    If[deg == 0,
      (
        result = {1}
      ),
      (
        If[minVar == maxVar,
          (
            result = {xminVardeg};
          ),
          (
            result =
              Flatten[Table[xminVardeg-i * allDegMonoms[i, maxVar, minVar + 1], {i, 0, deg}], 1];
          )];
      ]];
  result
)];
```

Example:

```
In[ ]:= allDegMonoms[5, 3, 1]
```

```
Out[ ]:= {x15, x14 x2, x14 x3, x13 x22, x13 x2 x3, x13 x32, x12 x23, x12 x22 x3, x12 x2 x32, x12 x33,
  x1 x24, x1 x23 x3, x1 x22 x32, x1 x2 x33, x1 x34, x25, x24 x3, x23 x32, x22 x33, x2 x34, x35}
```

A function to compute the degree of a monomial.

```
In[ ]:= degOfMon[mon_, varList_] := Module[{result, i, j, expLst},
  (
    expLst = Table[Exponent[mon, xi], {i, 1, Length[varList]}];
    result = Apply[Plus, expLst]
  )];
```

```
In[ ]:= degOfMon[1, {x1, x2, x3}]
```

```
Out[ ]:= 0
```

The next function sorts a list of monomials in  $x_1, \dots, x_n$  into decreasing lex order, degree by degree.

This function makes use of the fact that the built-in *Mathematica* function **MonomialList** returns the list of monomials using a monomial order that can be specified. The function first adds the monomials

in the list together and then applies **MonomialList** to this sum. We use the monomial order option **NegativeDegreeLexicographic** to generate the list in decreasing lex order, degree-by-degree, with the degrees increasing. If the input set of monomials is empty, the set {0} is returned.

```
In[ ]:= sortInLexOrder[monLst_, varLst_] :=
  MonomialList[Apply[Plus, monLst], varLst, NegativeDegreeLexicographic];

In[ ]:= sortInLexOrder[{x1, x22 x4, x3 x5, x43, x1 x52}, {x1, x2, x3, x4, x5}]

Out[ ]:= {x1, x3 x5, x1 x52, x22 x4, x43}

In[ ]:= sortInLexOrder[{ }, {x1, x2, x3, x4, x5}]

Out[ ]:= {0}
```

The next function **coeffOfTerm** extracts the (scalar) coefficient of a given monomial in a given polynomial.

Here is an example of *Mathematica*'s built-in **Coefficient** function in action:

```
In[ ]:= Coefficient[x1 - x23 - (x13 - 7) ^ 2 + 8 x3 + 3 x1 x3 - 2 x2 x32, x3]

Out[ ]:= 8 + 3 x1
```

Note that when applied to a list of polynomials, the list of coefficients is returned.

```
In[ ]:= Coefficient[{x, x y, x z}, x]

Out[ ]:= {1, y, z}
```

To extract the coefficient of the desired monomial (in the example,  $x_3$ ) only, and not have the “variable coefficients” such as  $3 x_1$  included. To achieve this behavior, we can use the following function that returns the output of **Coefficient** after substituting 0 into each of the variables; it also handles the special case of the monomial 1.

```
In[ ]:= coeffOfTerm[poly_, mon_, varList_] := Module[{result, nullSubs},
  (
    nullSubs = makeNullSubLst[varList] ;
    If[(mon /. nullSubs) == 0,
      result = Coefficient[poly, mon] /. nullSubs, result = poly /. nullSubs];
    result
  )]
```

Examples:

```
In[ ]:= varList

Out[ ]:= {x1, x2, x3}

In[ ]:= coeffOfTerm[x1 - x23 - (x13 - 7) ^ 2 + 8 x3 + 3 x1 x3 - 2 x1 x32, x1 x3, varList]

Out[ ]:= 3
```

```
In[ ]:= coeffOfTerm[x1 - x23 - (x13 - 7) ^ 2 + 8 x3 + 3 x1 x3 - 2 x2 x32, 1, varList]
Out[ ]:= -49
```

The following function takes a polynomial “poly” (in  $x_1 \dots x_n$ ) and a list of monomials “targetMonomLst,” and constructs the list of coefficients that each of the target monomials has in poly.

```
In[ ]:= makeCoeffLst[poly_, targetMonomLst_, varList_] :=
  Table[coeffOfTerm[poly, targetMonomLst[[i]], varList], {i, 1, Length[targetMonomLst]}];
```

The next function generalizes the preceding. It accepts a list of polynomials “polyLst” and the targetMonomLst, and constructs the list of the coefficient lists corresponding to the polynomials in polyLst.

```
In[ ]:= makeListOfCoeffLsts[polyLst_, targetMonomLst_, varList_] :=
  Table[makeCoeffLst[polyLst[[i]], targetMonomLst, varList], {i, 1, Length[polyLst]}];
```

The next function returns the index in the given list where the given item occurs (assuming the item appears once in the list). One has to be careful using this, as the “item” might be present as part of another item in the list, but not present as the item in itself. For example, if  $x_1 x_5^2$  is in a list but  $x_5^2$  is not, `indexOf` will still find it.

```
In[ ]:= indexOf[item_, lst_] := Position[lst, item][[1]][[1]];
```

```
In[ ]:= indexOf[9, Table[i^2, {i, 1, 5}]]
```

```
Out[ ]:= 3
```

```
In[ ]:= Position[{1, 2}, 3]
```

```
Out[ ]:= {}
```

```
In[ ]:= indexOf[x22, {x1, x1 x22}]
```

```
Out[ ]:= 2
```

The next function returns True if monomial  $m_1$  divides monomial  $m_2$ , and False otherwise.

```
In[ ]:= monomDivides[m1_, m2_, varList_] :=
Module[{exponentList1, exponentList2, result, okSoFar, i, numVars},
(
  numVars = Length[varList];
  exponentList1 = Table[Exponent[m1, varList[[i]]], {i, 1, numVars}];
  exponentList2 = Table[Exponent[m2, varList[[i]]], {i, 1, numVars}];
  okSoFar = True;
  i = 1;
  While[okSoFar && (i ≤ numVars),
    (
      okSoFar = exponentList1[[i]] ≤ exponentList2[[i]];
      i = i + 1;
    )];
  result = okSoFar;
  result
)];
```

```
In[ ]:= monomDivides[x2 x3, x13 x2 x32, {x1, x2, x3}]
```

```
Out[ ]:= True
```

```
In[ ]:= monomDivides[x13, x12, {x1, x2}]
```

```
Out[ ]:= False
```

The next functions return the head and the tail of a given arrow  $A \rightarrow B$ .

```
In[ ]:= head[a_ → b_] := a;
tail[a_ → b_] := b;
```

The next function computes the product of two ideals by multiplying each generator of the first into each generator of the second. Each input ideal is a list of its generators.

Q: why did I include varList as a parameter? Perhaps I wanted to order the result in a certain way??

```

In[ ]:= idealProd[id1_, id2_, varList_] := Module[{result, i, j, len1, len2},
  (
    len1 = Length[id1];
    len2 = Length[id2];
    result = {};
    For[i = 1, i ≤ len1, i++,
      (
        For[j = 1, j ≤ len2, j++,
          (
            result = Append[result, id1[[i]] * id2[[j]]];
          )];
        DeleteDuplicates[result]
      )];
  );

In[ ]:= varList
Out[ ]:= {x1, x2, x3}

In[ ]:= idealProd[{x1, x1 x2, x22 - x1 x2}, {x2, x2 x3, x3}, varList]
Out[ ]:= {x1 x2, x1 x2 x3, x1 x3, x1 x22, x1 x22 x3, x2 (-x1 x2 + x22), x2 (-x1 x2 + x22) x3, (-x1 x2 + x22) x3}

```

We now extend the previous function to a function to compute the product of a list of ideals. We assume that the list is of length at least 1.

```

In[ ]:= prodOfIdeals[idealList_, varList_] := Module[{result, numIdeals, i},
  (
    numIdeals = Length[idealList];
    result = idealList[[1]];
    For[i = 2, i ≤ numIdeals, i++,
      (
        result = idealProd[result, idealList[[i]], varList];
      )];
    result
  );

In[ ]:= varList
Out[ ]:= {x1, x2, x3}

In[ ]:= prodOfIdeals[{ {x1, x1 x2, x22 - x1 x3}, {x2, x2 x3, x3}, {x3 x4} }, varList ]
Out[ ]:= {x1 x2 x3 x4, x1 x2 x32 x4, x1 x32 x4, x1 x22 x3 x4, x1 x22 x32 x4,
  x2 x3 (x22 - x1 x3) x4, x2 x32 (x22 - x1 x3) x4, x32 (x22 - x1 x3) x4}

```

## II. Utilities for General Border Bases and Border Pre-Bases

The next function constructs the set of boundary monomials associated to a

given order ideal (entered as a list of monomials called “basis”) in the variables of varList.

```
In[*]:= bdryMonoms[basis_, varList_] := Module[{result, i, j, numBasis, curMon, curMonInBasis, n},
  (
    n = Length[varList];
    numBasis = Length[basis];
    result = {};

    For[i = 1, i ≤ n, i++,
      (
        For[j = 1, j ≤ numBasis, j++,
          (
            curMon = varList[[i]] * basis[[j]];
            curMonInBasis = MemberQ[basis, curMon];
            If[! curMonInBasis, result = Append[result, curMon]];
          )];
        )];
    result = sortInLexOrder[DeleteDuplicates[result], varList]
  )];
```

Example:

```
In[*]:= bdry = bdryMonoms[{1, x1, x2, x3, x2 x3, x32, x33}, {x1, x2, x3}]
```

```
Out[*]:= {x12, x1 x2, x1 x3, x22, x1 x2 x3, x1 x32, x22 x3, x2 x32, x1 x33, x2 x33, x34}
```

The following function takes a polynomial that is a linear combination of basis and boundary monomials (typical case: an S-polynomial of two members of a border basis or pre-basis), and reduces the polynomial modulo the border basis/pre-basis. The result is a linear combination of basis monomials only.

**The following code depends for its correctness on having the border basis list (“borBasis”) in the same order as the list of boundary monomials (“bdry”).** The first input “poly” is a polynomial that is a linear combination of basis and boundary monomials. The output is the polynomial reduced modulo the border basis (which is accordingly a linear combination of basis monomials only). This is not a fully general reduction procedure, but it is all we need for computing linear syzygies and the tangent space relations associated to a basis of linear syzygies.

```

In[ ]:= reducePoly[poly_, bdry_, borBasis_, varList_] := Module[{result, curCoeff, numBdry, i},
  (
    result = poly;
    numBdry = Length[bdry];

    For[i = 1, i ≤ numBdry, i++,
      (
        curCoeff = coeffOfTerm[result, bdry[[i]], varList];
        result = result - curCoeff * borBasis[[i]];
      )];
    result
  )];

```

The next function generalizes the preceding one, and allows us to reduce the product of a monomial times a linear combination of basis and boundary monomials. It does this by doing an initial reduction, and then multiplying the linear combination by one variable in the monomial at a time, and reducing. The monomial is entered as a list of its variable factors, for example,  $x_1^2 x_3 x_4^3$  could be entered as any rearrangement of the list  $\{x_1, x_1, x_3, x_4, x_4, x_4\}$ .

```

In[ ]:= basisLinCombTimesMonom[linComb_, mon_, bdry_, borBasis_, varList_] :=
  Module[{curVar, monDeg, result, i},
    (
      monDeg = Length[mon];
      result = reducePoly[linComb, bdry, borBasis, varList];
      (* linComb only involves basis and bdry monomials *)
      For[i = 1, i ≤ monDeg, i++,
        (
          curVar = mon[[i]];
          result = reducePoly[result * curVar, bdry, borBasis, varList];
          (* result*curVar has at worst boundary monomials *)
        )];
      result
    )];

```



The next function constructs a basis of the linear syzygies of the given border Basis. It implements the algorithm described in Section 2.3 of the paper “Some Elementary Components of the Hilbert Scheme of Points.”

```

In[ ]:= makeLinearSyzygies[bdry_, borBasis_, varList_] :=
Module[{numBdry, result, i, j, p, z, T, numTargets, multipliers, numMultipliers,
  products, numProducts, theMatrix, nulSp, curMonSyz, curCoeff, numVars},
(
  numVars = Length[varList];
  numBdry = Length[bdry];

  (* We next form the set T of "target monomials" as described in Section 2.3 *)
  T = DeleteDuplicates[
    Join[bdry, Flatten[Table[varList[[i]] * bdry[[j]], {i, 1, numVars}, {j, 1, numBdry}]]];
  numTargets = Length[T];

  (* The set "products" is the set of
    images of the basis elements  $e_{\{\alpha, j\}}$  of the vector space E *)
  multipliers = Join[{1}, varList];
  numMultipliers = numVars + 1;
  products = Flatten[
    Table[multipliers[[i]] * borBasis[[j]], {i, 1, numMultipliers}, {j, 1, numBdry}]];
  numProducts = numBdry * numMultipliers;

  (* "theMatrix is the matrix
    of the map  $\sigma$  with respect to the bases  $\{e_{\{\alpha, j\}}\}$  and T *)
  theMatrix = Transpose[makeListOfCoeffLsts[products, T, varList]];
  (* This matrix must have maximal rank = numTargets,
  since the map  $\sigma$  is surjective *)

  nulSp = NullSpace[theMatrix]; (* This is a list of length
    (numProducts - numTargets) consisting of lists of length numProducts *)

  (* Now we must assemble the syzygies corresponding to each of the lists in nulSp *)
  (* This list "result" is the output of the function. *)

  result = {};
  For[p = 1, p ≤ numProducts - numTargets, p++,
    ((* Extract the pth monomial syzygy *)
    curMonSyz = Table[0, {i, 1, numBdry}];
    For[z = 1, z ≤ numProducts, z++,
      (
        curCoeff = nulSp[[p]][[z]];
        i = Quotient[z - 1, numBdry] + 1;
        j = Mod[z - 1, numBdry] + 1;
        curMonSyz[[j]] = curMonSyz[[j]] + curCoeff * multipliers[[i]];
      );
    result = Append[result, curMonSyz];
  ];

  result

)];

```

The next function generates the generic border pre-basis, given the basis set and the boundary set. The functionality of this function was coded “in-line” in the function that follows this one.

```

In[ ]:= genericBorderPreBasis[basis_, bdry_] := Module[{i, j, numBasis, numBdry},
  (
    numBasis = Length[basis];
    numBdry = Length[bdry];
    Table[bdry[[j]] -  $\sum_{i=1}^{\text{numBasis}} C_{\{i,j\}} \text{basis}[[i]]$ , {j, 1, numBdry}]
  )];

```

The next function constructs the generators of the ideal of the border basis scheme (denoted  $\phi_i^{j,j'}$  in Section 2.4 of the paper). This is done by computing the reduced S-polynomials  $\bar{S}(G_j, G_{j'})$  relative to the “generic O-border pre-basis”  $\{G_j\}$  and extracting the coefficients of each of the basis monomials.

```
ln[ ]:= makeBorBasisSchemeIdealGenerators[basisSet_, varList_] :=
Module[{result, i, j, bdry, numBdry, numBasis, genericBorderPreBasis, linearMonomialSyz,
  genericLinearSyzLst, bdrySyzAppliedToGenericPreBasis, lstOfReducedSPolys, numSyz},
(
  bdry = bdryMonoms[basisSet, varList];
  numBdry = Length[bdry];
  numBasis = Length[basisSet];
  genericBorderPreBasis =
    Table[bdry[[j]] -  $\sum_{i=1}^{\text{numBasis}} C_{\{i,j\}} \text{basisSet}[[i]], \{j, 1, \text{numBdry}\}$ ];
  (* We now find a basis of the linear syzygies of the boundary monomials *)
  linearMonomialSyz = makeLinearSyzygies[bdry, bdry, varList];

  numSyz = Length[linearMonomialSyz];

  (* Construct list of generic linear
    syzygies from the syzygies of the boundary monomials *)

  genericLinearSyzLst = {};
  For[i = 1, i ≤ numSyz, i++,
    (
      bdrySyzAppliedToGenericPreBasis = genericBorderPreBasis.linearMonomialSyz[[i]];
      genericLinearSyzLst = Append[genericLinearSyzLst, linearMonomialSyz[[i]] -
        makeCoeffLst[bdrySyzAppliedToGenericPreBasis, bdry, varList]];
    );
  ];

  lstOfReducedSPolys =
    Table[genericLinearSyzLst[[i]].genericBorderPreBasis, {i, 1, numSyz}];
  result = Flatten[makeListOfCoeffLsts[lstOfReducedSPolys, basisSet, varList]];
  result
)];
```

The next function makes a list of the generic neighbor syzygies, given the basis set and the list of variables. The functionality of this function was coded “in-line” in the preceding function, but it is sufficiently useful that we decided to pull it out as a separate function.

```

In[ ]:= makeGenericNeighborSyzygies[basisSet_, varList_] :=
Module[{result, i, j, bdry, numBdry, numBasis, genericBorderPreBasis, linearMonomialSyz,
  genericLinearSyzLst, bdrySyzAppliedToGenericPreBasis, lstOfReducedSPolys, numSyz},
(
  bdry = bdryMonoms[basisSet, varList];
  numBdry = Length[bdry];
  numBasis = Length[basisSet];
  genericBorderPreBasis =
    Table[bdry[[j]] -  $\sum_{i=1}^{\text{numBasis}} c_{\{i,j\}}$  basisSet[[i]], {j, 1, numBdry}];
  (* We now find a basis of the linear syzygies of the boundary monomials *)
  linearMonomialSyz = makeLinearSyzygies[bdry, bdry, varList];

  numSyz = Length[linearMonomialSyz];

  (* Construct list of generic linear
    syzygies from the syzygies of the boundary monomials *)

  genericLinearSyzLst = {};
  For[i = 1, i ≤ numSyz, i++,
    (
      bdrySyzAppliedToGenericPreBasis = genericBorderPreBasis.linearMonomialSyz[[i]];
      genericLinearSyzLst = Append[genericLinearSyzLst, linearMonomialSyz[[i]] -
        makeCoeffLst[bdrySyzAppliedToGenericPreBasis, bdry, varList]];
    );
  genericLinearSyzLst
)];

```

The next function generates a list of the indeterminates  $C_{\{i,j\}}$  that are the coefficients in the generic O-border pre-basis.

```

In[ ]:= makeCLst[numBasis_, numBdry_] := Flatten[Table[C_{i,j}, {j, 1, numBdry}, {i, 1, numBasis}]]

```

The next function takes a given border (pre)basis, and constructs the list of substitutions  $\{C_{\{i,j\}} \rightarrow c_{\{i,j\}}\}$  that correspond to it. It is assumed that the border

(pre)basis list is in the same order as the list of boundary monomials.

```
ln[ ]:= makeCCoordsOfBorBasis[borBasis_, basisSet_, bdry_, varList_] :=
Module[{numBasis, numBdry, result, listOfCs, i, j},
(
numBasis = Length[basisSet];
numBdry = Length[bdry];
result = {};

For[j = 1, j ≤ numBdry, j++,
(
For[i = 1, i ≤ numBasis, i++,
(
result =
Append[result, C{i,j} → -coeffOfTerm[borBasis[[j]], basisSet[[i]], varList] ];
)];
)];
result
)];
```

The next function reverses the previous one: it takes a list of substitutions  $\{C_{\{i,j\}} \rightarrow c_{\{ij\}}\}$  that define a point in the border basis scheme, and produces the corresponding border basis.

```
ln[ ]:= makeBorBasisCorrespToCCoords[subList_, basisSet_, bdry_] :=
Module[{i, j, numBasis, numBdry, ijIndex},
(
numBasis = Length[basisSet];
numBdry = Length[bdry];
Table[bdry[[j]] -  $\sum_{i=1}^{\text{numBasis}} C_{\{i,j\}} \text{basisSet}[[i]], \{j, 1, \text{numBdry}\}] /. \text{subList}$ 
)];
```

We now add the sigma and tau functions (and their “inverses”) from the rho syzygies paper of 2010. This might allow us to be more effective in exploring our rho syzygies computationally. (See page 4 of that paper. ) -- this functionality is not needed for the “More Elementary Components” paper.

The next function computes the members of the generic border pre-basis.

The next function gives us the list of F-polys, which have the form  $f_j = b_j - \sum_{i=1}^{\mu} C_{\{i,j\}} t_i$ , where the b's are the bdry monomials and the t's are the basis monomials.

```
ln[ ]:= fPolys[basis_, bdry_] := Module[{result, numBasis, numBdry},
  (
    numBasis = Length[basis];
    numBdry = Length[bdry];
    result = Table[bdry[[j]] -  $\sum_{i=1}^{\text{numBasis}} C_{\{i,j\}} \text{basis}[[i]]$ , {j, 1, numBdry}]
  )]
```

### III. Functions for computing tangent space dimensions at points [I] such that I has a border basis.

The next function constructs a list of all tangent space relations associated to a basis of linear syzygies (which generate the complete syzygy module) of the border basis of  $I$ .

Recall that each syzygy gives rise to  $\mu$  relations, one for each monomial in the order ideal (or basis set). The function returns a tuple containing {aLst, grandListOfTanSpaceRelns}, where aLst is a list of indeterminates  $a_{\{i,j\}}$  that represent the tuple of the “generic tangent vector,” and grandListOfTanSpaceRelns is the desired list of tangent space relations, which are represented as tuples of scalars  $(c_{\{i,j\}})$  such that  $(\sum_{\{i,j\}} c_{\{i,j\}} \cdot a_{\{i,j\}}) = 0$  for all tangent vectors, which are encoded as tuples of scalars  $(a_{\{i,j\}})$ , as explained in Section 4 of the “Some elementary components of the Hilbert scheme of points” paper.

```

In[*]:= makeTanSpaceReIns[borBasis_, basisSet_, bdry_, varList_] :=
Module[{result, tanVecLst, numBasis, numBdry, aLst, numAs, nbrSyzygies, numSyz, i, j, k, z,
  curSyz, syzAppliedToTanVec, coeffs, curTanSpaceReIns, grandListOfTanSpaceReIns},
(
  numBasis = Length[basisSet];
  numBdry = Length[bdry];
  n = Length[varList];

  (* tanVecLst is the list of images
    (v(g1), v(g2), ..., v(gv)) where v is a "generic tangent vector," gi
    are the border basis elements, and the images lie in basisSet. *)
  tanVecLst = Table[ $\sum_{i=1}^{\text{numBasis}} (a_{\{i,j\}} \text{basisSet}[[i]])$ , {j, 1, numBdry}];
  aLst = Flatten[Table[a_{i,j}, {j, 1, numBdry}, {i, 1, numBasis}]];
  numAs = Length[aLst];
  nbrSyzygies = makeLinearSyzygies[bdry, borBasis, varList];
  numSyz = Length[nbrSyzygies];

  grandListOfTanSpaceReIns = {};

  For[z = 1, z ≤ numSyz, z++,
    (* For each syzygy, find the associated tangent space relations, and add them to
      the growing list of these. We do this by applying the syzygy to tanVecLst,
      reducing modulo the borBasis, and finding the coefficients of the basis monomials
      in the resulting expression (which must be 0 modulo the border basis). *)
    curSyz = nbrSyzygies[[z]];
    syzAppliedToTanVec = reducePoly[curSyz.tanVecLst, bdry, borBasis, varList];
    coeffs = makeCoeffLst[syzAppliedToTanVec, basisSet, varList];
    curTanSpaceReIns =
      Table[Coefficient[coeffs[[j]], aLst[[k]]], {j, 1, numBasis}, {k, 1, numAs}];
    grandListOfTanSpaceReIns = Join[grandListOfTanSpaceReIns, curTanSpaceReIns];
  ];

  result = {aLst, grandListOfTanSpaceReIns}
)];

```



The next function finds the dimension of the tangent space at the point  $[/]$ . We assume that the user has separately executed the **makeTanSpaceReIns** function to obtain the  $aLst$  and list of  $tanSpReIns$

```
In[ ]:= tanSpaceDim[aLstLength_, tanSpReIns_] := Module[{result, rankOfReIns},
  (
    rankOfReIns = MatrixRank[tanSpReIns];
    result = aLstLength - rankOfReIns;
    result
  )];

In[ ]:= tanSpaceDim[aLstLength_, tanSpReIns_, modulus_] := Module[{result, rankOfReIns},
  (
    rankOfReIns = MatrixRank[tanSpReIns, Modulus -> modulus];
    result = aLstLength - rankOfReIns;
    result
  )];
```

---

## IV. Functions for constructing the various sets and parameters associated with distinguished and mod-distinguished ideals.

### 1. makeBasisAndBoundaryMonomialLists

Given the “signature” of the example being studied, this function constructs and returns the lists of basis and boundary monomials in negative degree-lex order, in which higher-degree monomials follow lower-degree monomials. The parameters are  $(n, r, s, \delta, w)$  -- the entries in the signature, as defined in the paper. The function computes and returns the lists of basis and boundary monomials, the Hilbert function, the leading monomials LM, the trailing monomials TM, the sets  $\mathcal{T} = \text{Tar}$  and  $\text{Tar}'$ , and the parameters  $\mu = |\text{basis}|$ ,  $\nu = |\text{bdry}|$ ,  $\lambda = |\text{LM}|$ , and  $\tau = |\text{TM}|$ .

```
In[ ]:= makeBasisAndBoundaryMonomialLists[n_, r_, s_, delta_, w_] :=
  Module[{varList, mons, basis, bdry, basisMonLst, bdryMonLst,
    minLM, minLMIndex, minMonDegd, minMonDegdIndex, HilbertFunction, i,
    j, k, d, mu, nu, ell, tau, LM, TM, TarPrime, Tar, startIndex, endIndex},
    (
      varList = Table[x_i, {i, 1, n}];

      mons = Table[{}, {i, 1, s + 1}];
      basis = {};
      bdry = {};
      HilbertFunction = {1};

      (* First create lists of all monomials of degree d, 0 ≤ d ≤ s+1 *)
```

```

basis = {1}; (* The lone element of degree 0. *)

For[d = 1, d ≤ s + 1, d++,
(
  mons[[d]] = allDegNMonoms[d, n, 1];
)];

(* Add all the monomials of degrees 1 ≤ d < r to the basis,
and update HilbertFunction. *)
For[d = 1, d ≤ r - 1, d++,
(
  basis = Join[basis, mons[[d]]];
  HilbertFunction = Append[HilbertFunction, Length[mons[[d]]]];
)];

(* Next add the basis monomials of degrees r through s to the basis,
and update HilbertFunction. *)
minLM =  $x_\delta^{r-w} x_n^w$ ;
minLMIndex = indexOf[minLM, mons[[r]]];
basisMonLst = Take[mons[[r]], - (Length[mons[[r]]] - minLMIndex)];
basis = Join[basis, basisMonLst];
HilbertFunction = Append[HilbertFunction, Length[basisMonLst]];

minMonDegd = minLM;
For[d = r + 1, d ≤ s, d++,
(
  minMonDegd =  $x_n$  * minMonDegd;
  minMonDegdIndex = indexOf[minMonDegd, mons[[d]]];
  basisMonLst = Take[mons[[d]], - (Length[mons[[d]]] - minMonDegdIndex)];
  basis = Join[basis, basisMonLst];
  HilbertFunction = Append[HilbertFunction, Length[basisMonLst]];
  If[d == s,
  (
    TM = basisMonLst; (* The trailing monomials. *)
  )];
)];

(* At this point "basis" is the full list of all basis elements *)

(* Next,
we will construct the target sets "TarPrime" and "Tar," the former first: *)
(* The lex-maximal basis monomial of degree r is  $x_\delta^{r-(w+1)} x_{\delta+1}^{w+1}$ ,
and the lex-min bdry mon of degree s-1 is  $x_n^{s-1}$ . *)
(* The lex-min element of Tar has index Length[basis] =  $\mu$ , of course. *)
startIndex = indexOf[ $x_\delta^{r-(w+1)} x_{\delta+1}^{w+1}$ , basis];
endIndex = indexOf[ $x_n^{s-1}$ , basis];
TarPrime = Take[basis, {startIndex, endIndex}];
Tar = Take[basis, {startIndex, Length[basis]}];

(* Next we create the list of boundary monomials. We begin with
the leading monomials LM, the boundary monomials of degree r. *)

```

```

LM = Take[mons[[r]], minLMIndex];
bdry = Join[bdry, LM];

(* Next we add the boundary monomials of degrees r+1 through s. *)
For[d = r + 1, d ≤ s, d++,
(
  basisMonLst = Take[mons[[d - 1]], -HilbertFunction[[d]]];
  (* Basis mons of one less degree. *)
  bdryMonLst = sortInLexOrder[DeleteDuplicates[
    Flatten[Table[Complement[xk * basisMonLst, basis], {k, 1, n}]]], varList];
  bdry = Join[bdry, bdryMonLst];
)];

(* Finally we add the boundary monomials of degree s+1,
all the "variable*TM" products. *)
bdryMonLst = sortInLexOrder[DeleteDuplicates[
  Flatten[Table[xk * TM, {k, 1, n}]]], varList];
bdry = Join[bdry, bdryMonLst];

(* Return the results. *)
μ = Length[basis]; (* Total number of basis monomials *)
ν = Length[bdry];
ell = Length[LM];
τ = Length[TM];

{basis, bdry, HilbertFunction, LM, TM, TarPrime, Tar, μ, ν, ell, τ}
)];

```

2. The following function computes the size of the set  $|\Theta|$ , which is the number of parameters  $\theta_q$  that define the initial generic target assignment.

$$\text{In}[*]:= \text{numThetas}[n\_ , r\_ , s\_ , \text{delta}\_ , w\_ ] := \sum_{d=r}^{s-1} \left( \sum_{e=d-(r-(w+1))}^d \left( \sum_{u=0}^{e-w} \text{Binomial}[u + (n - \text{delta} - 1) - 1, u] \right) \right)$$

```

In[*]:= numThetas[5, 2, 3, 3, 0]

```

```

Out[*]= 5

```

3. The following function computes the monomials in tarPrime that are divisible by  $x_{\delta+1}^w$ , which will be the ones that appear in the initial generic target. (There are numThetas of them.)

We simply run through the list tauPrime and make the list of those that are divisible by  $x_{\delta+1}^w$ .

```

In[*]:= varList = Table[xi, {i, 1, n}];

```

```

In[*]:= varList

```

```

Out[*]= {x1, x2, x3}

```

```

ln[*]:= initialTargetMons[tarPrime_, n_,  $\delta$ _, w_] := Module[{i, j, result, lenTarPrime, varList},
  (
    lenTarPrime = Length[tarPrime];
    varList = Table[xi, {i, 1, n}];
    result = {};
    For[i = 1, i ≤ lenTarPrime, i++,
      (
        If[monomDivides[x $\delta$ +1w, tarPrime[[i]], varList],
          (
            result = Append[result, tarPrime[[i]]];
          )];
      )];
    result
  )];

```

4. The following function computes  $\dim(U) = \text{ell} * \tau + \gamma + (\delta - 1) * \eta + (n - \delta + 1)$  -- this is equation (54) in the paper.

Here  $\gamma = \text{numThetas} = \#$  monomials in tarPrime that are divisible by  $x_{\delta+1}^w$ . We have that. We need one more parameter, namely the value of  $\eta$ . Recall that  $\eta = |\Delta_\alpha|$  for  $1 \leq \alpha < \delta$  (see section 11.1 of the paper). The value of  $\eta$  is equal to

$$\begin{aligned}
 & 1 + |\{\text{monomials } m \in k[x_\delta, \dots, x_n] : m \cdot x_n^{r-1} \in \text{tarPrime}\}| \\
 & = 1 + |\{\text{monomials } m \in k[x_\delta, \dots, x_n] : 1 \leq \deg(m) \leq s - r \text{ and } x_\delta - \deg(m) < r - \delta\}|
 \end{aligned}$$

where the leading summand of 1 is to count the monomial  $m = 1$ .

Here is the pseudocode for the function:

```

result = 0;
For each possible power d of x $\delta$  from 0 through r - (w + 1), DO
  For each possible power e of a monomial in x $\delta$ +1 ... xn from 0 to s - r - d, DO
    result = result + # monomials in x $\delta$ +1 ... xn of degree e = result +  $\binom{n - \delta - 1 + e}{e}$ ;
  end For_e
End For_d
return result =  $\eta$ .

```

```

In[ ]:= findEta[n_, r_, s_, δ_, w_] := Module[{result, d, e},
  (
    result = 0;
    For[d = 0, d ≤ r - (w + 1), d++,
      (
        For[e = 0, e ≤ s - r - d, e++,
          (
            result = result + Binomial[n - δ - 1 + e, e];
          )];
        )];
    result
  )];

```

```

In[ ]:= findEta[r, 3, 4, 2, 1]

```

```

Out[ ]:= 3

```

5. The following function returns  $\dim(U)$ , using the formula of equation (54) of the paper.

$$\dim(U) = \text{ell} \cdot \tau + \gamma + (\delta - 1) \eta + (n - \delta + 1)$$

```

In[ ]:= findDimU[n_, r_, s_, δ_, w_, ℓ_, τ_] := Module[{result, η, γ},
  (
    γ = numThetas[n, r, s, δ, w];
    η = findEta[n, r, s, δ, w];
    result = ℓ * τ + γ + (δ - 1) * η + n - δ + 1
  )];

```

```

In[ ]:=

```
